# Supplementary material for: Compressible Latent-Space Invertible Networks for Generative Model-Constrained Image Reconstruction
Source: arXiv:2007.02462 source file (2020-12-30)

|              |                                                                                     |                                                                                     |                                                                                      |                                                                                       |
|--------------|-------------------------------------------------------------------------------------|-------------------------------------------------------------------------------------|--------------------------------------------------------------------------------------|---------------------------------------------------------------------------------------|
| PLS-TV       | $\lambda = 0.0040$<br>RMSE = 0.0257                                                 | $\lambda = 0.0100$<br>RMSE = 0.0256                                                 | $\lambda = 0.2626$<br>RMSE = 0.0236                                                  | $\lambda = 1.1602$<br>RMSE = 0.0250                                                   |
|              | 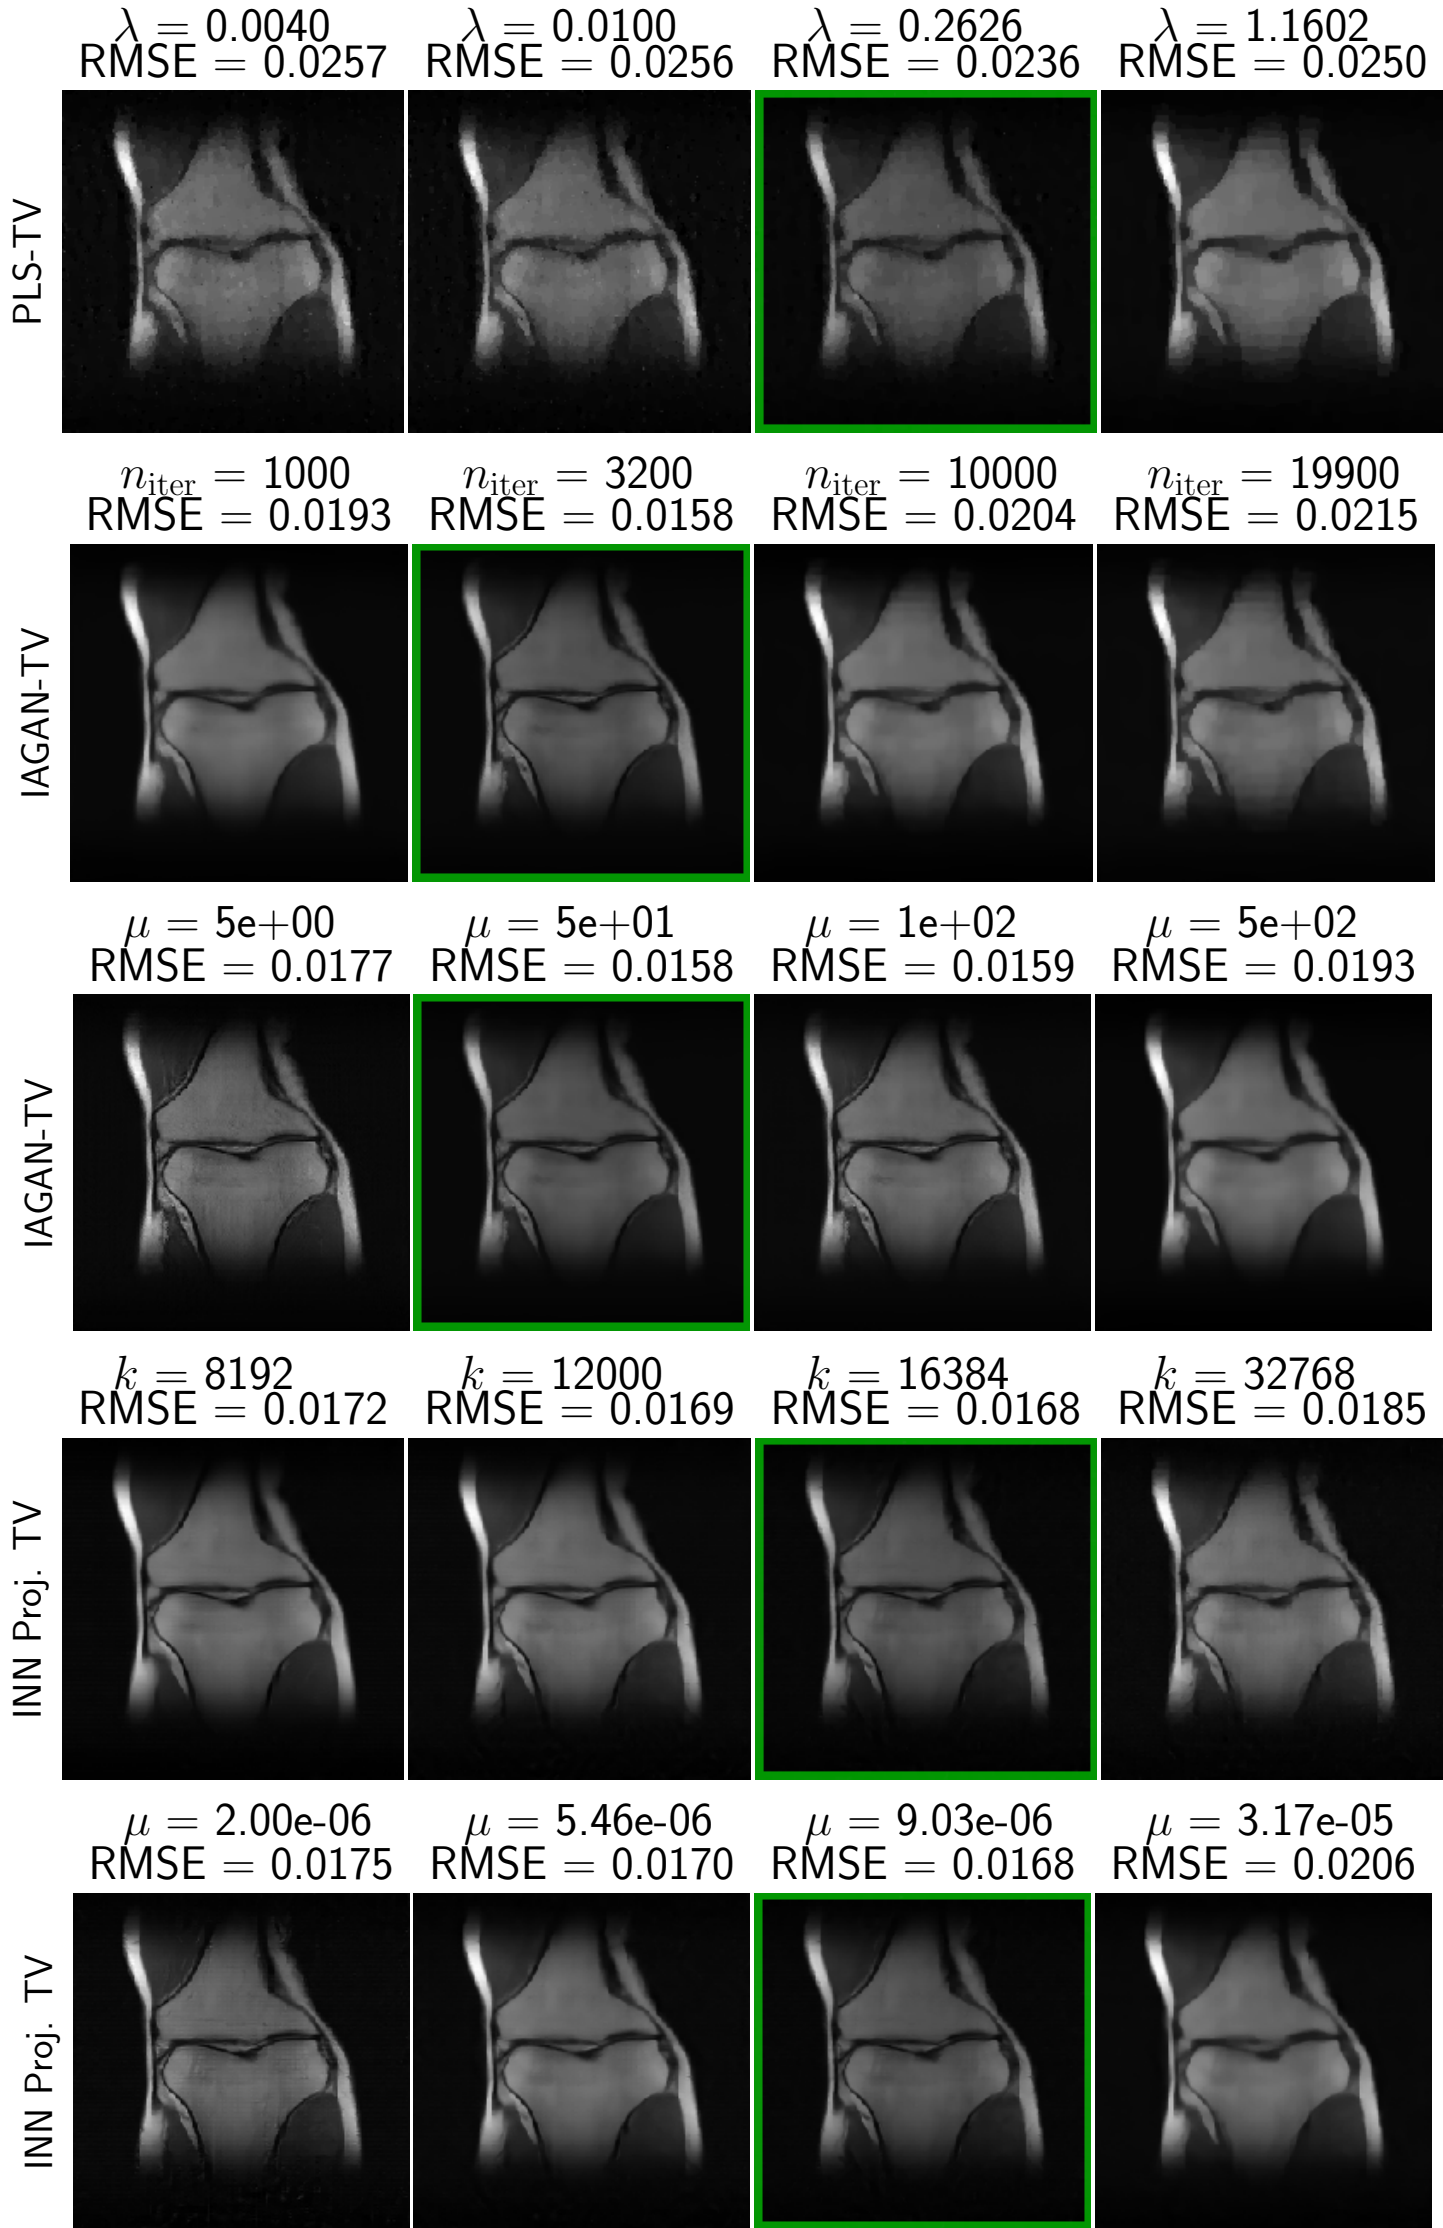    | 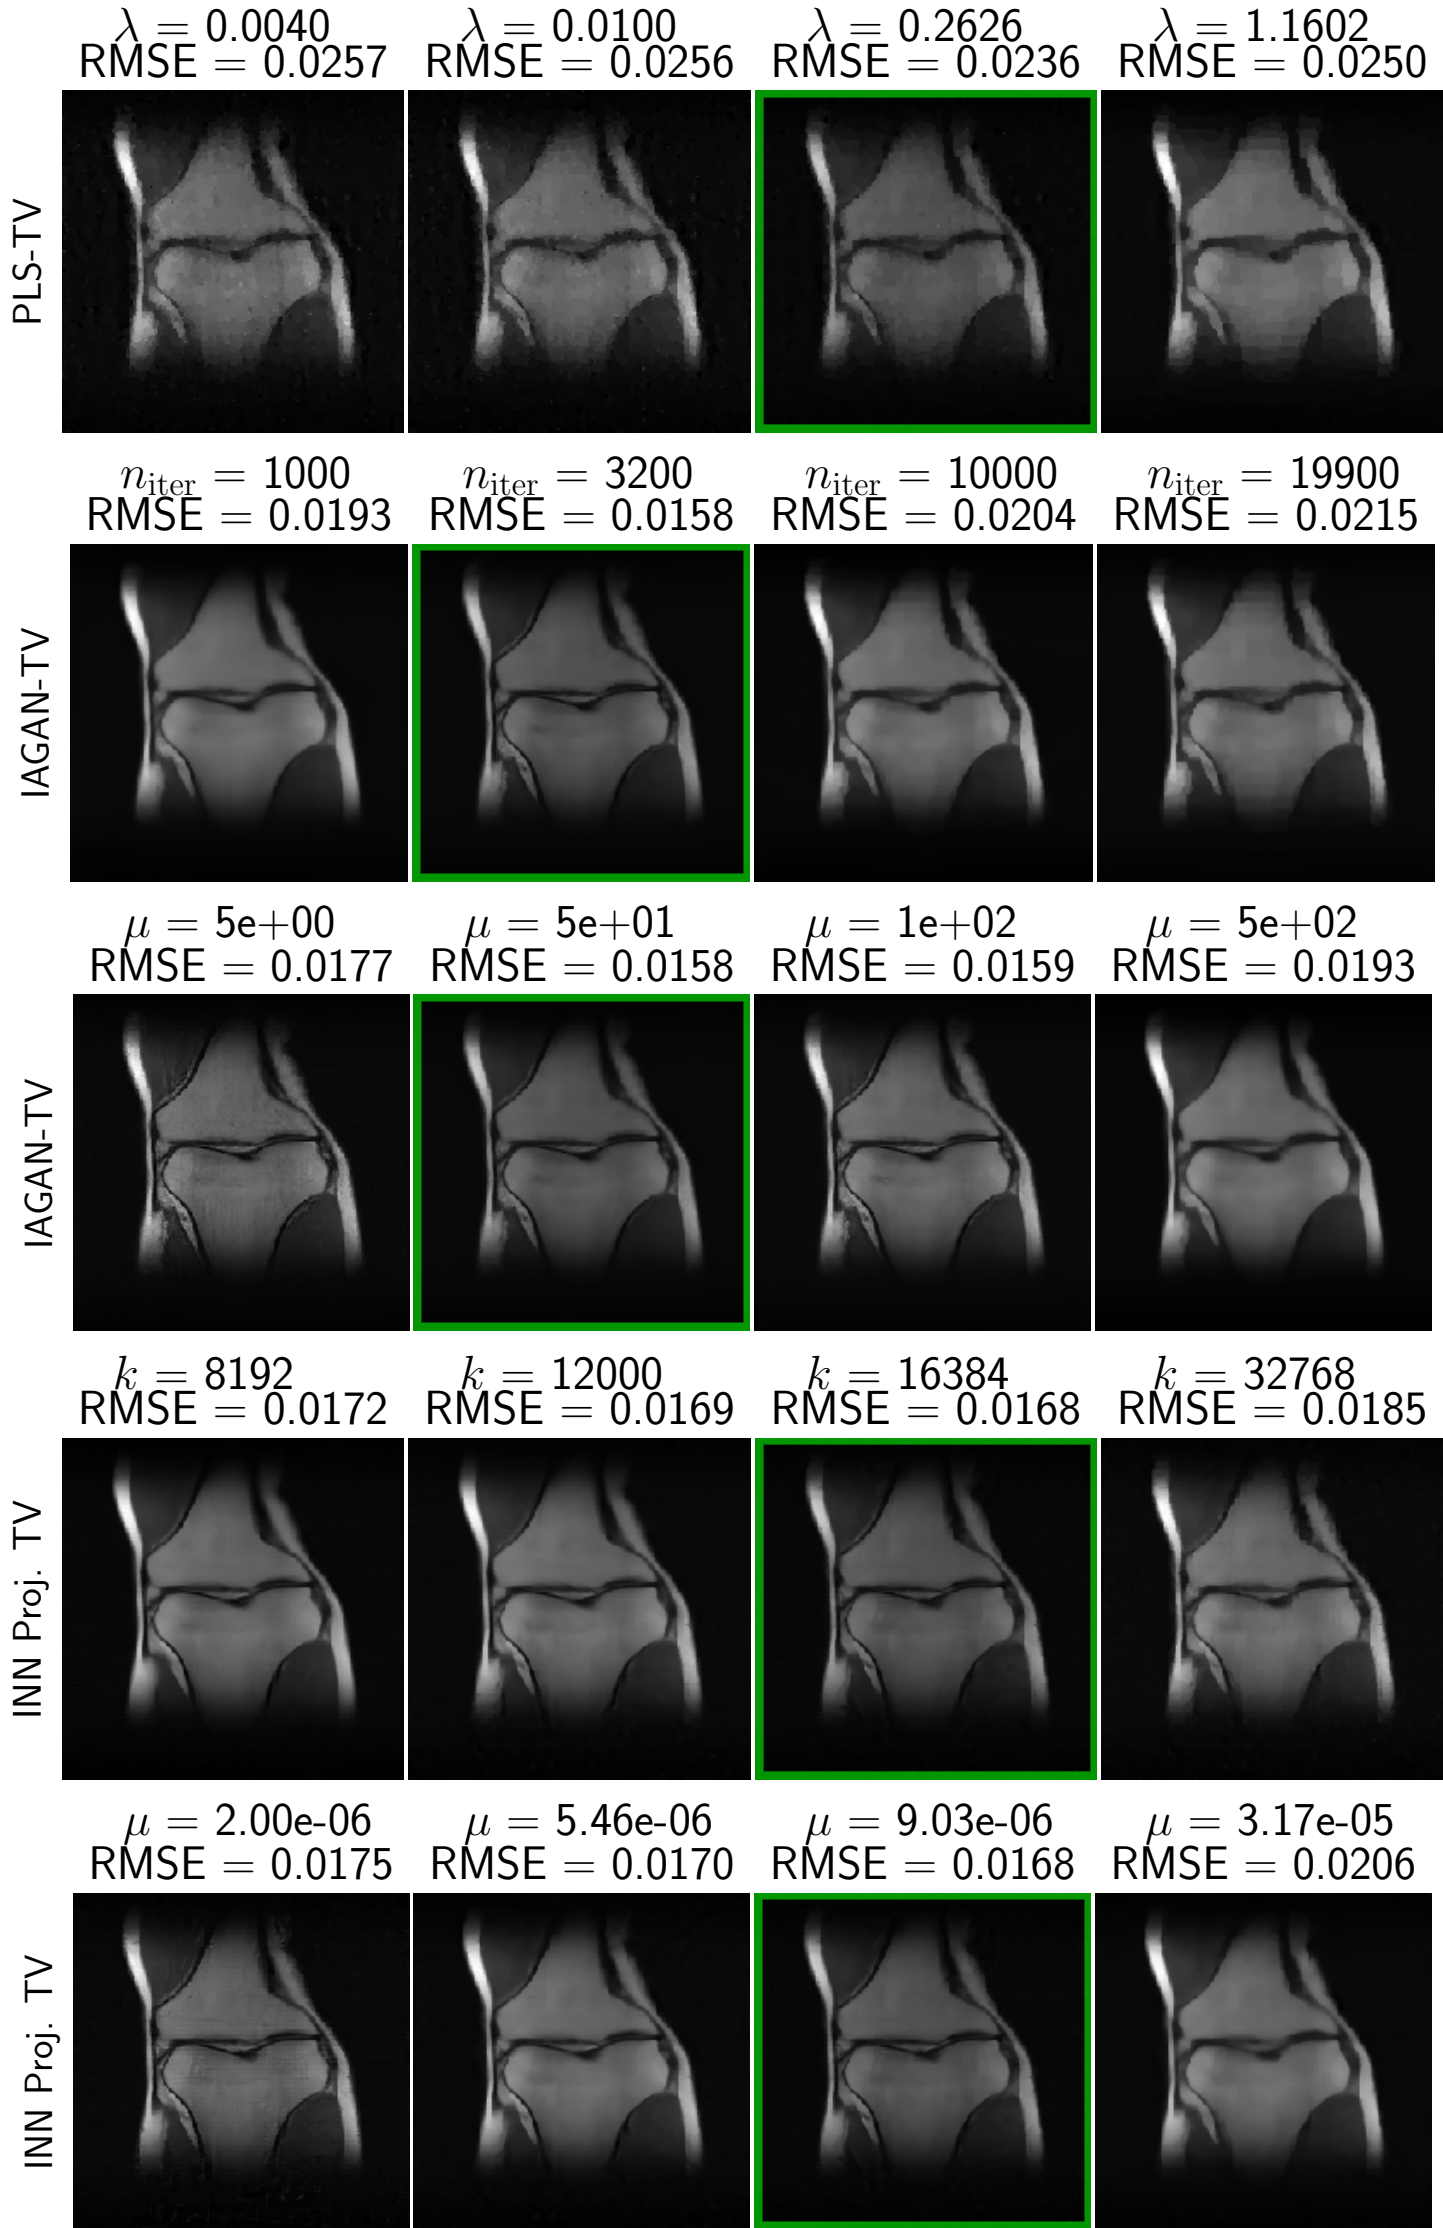    | 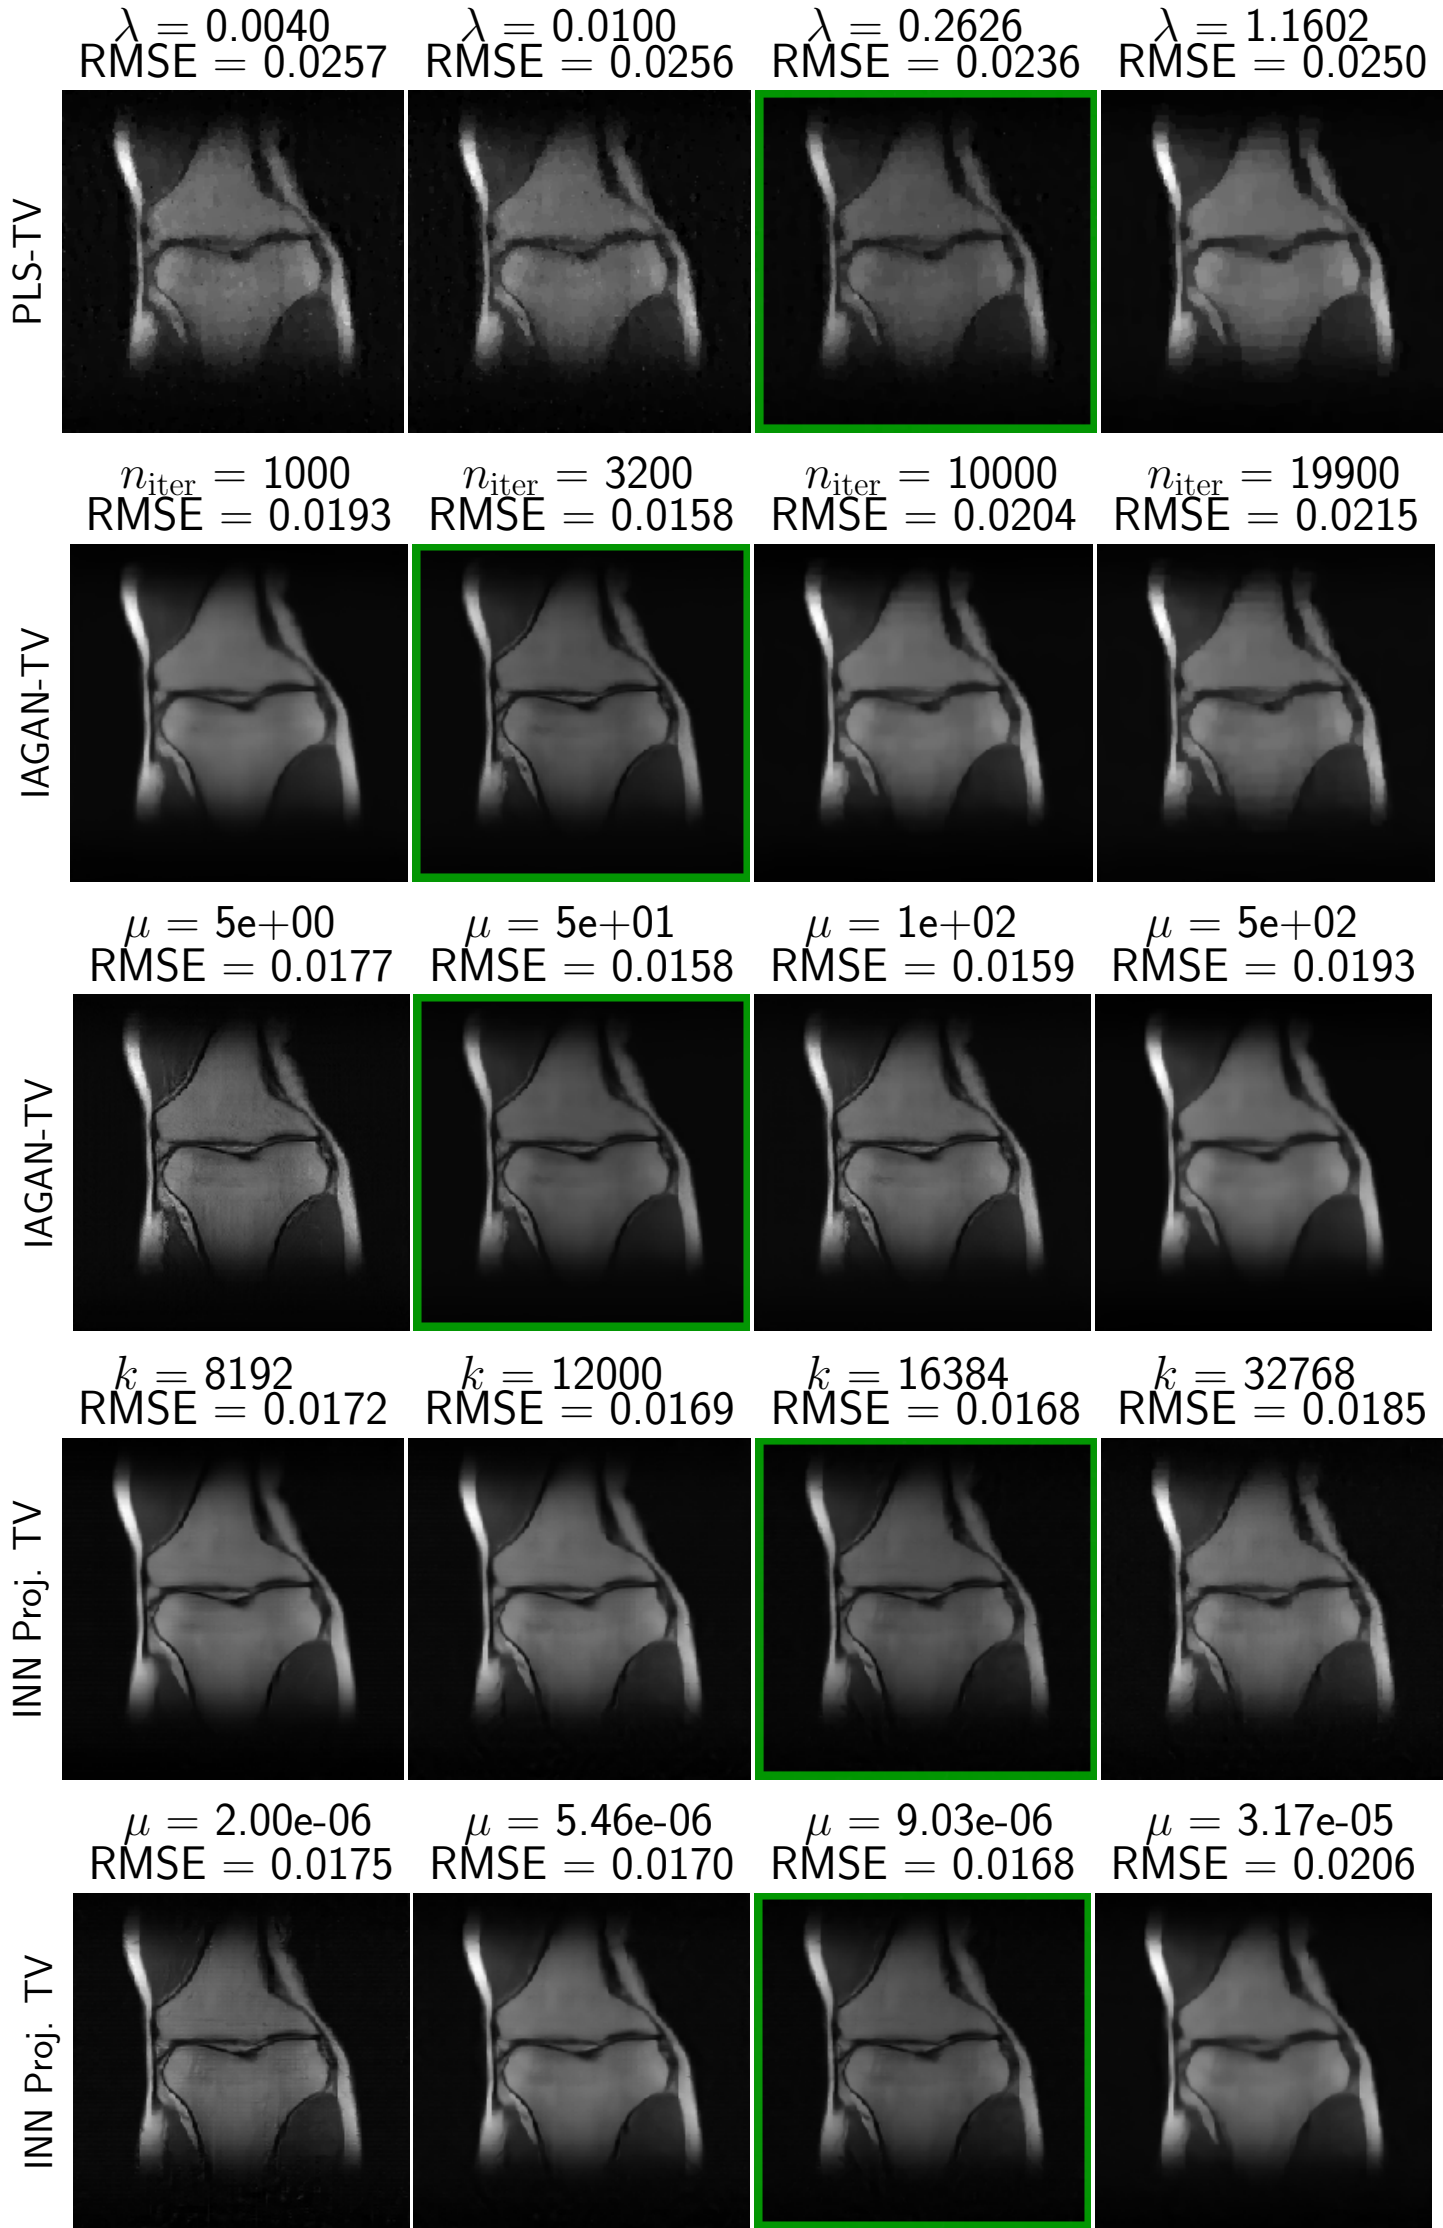    | 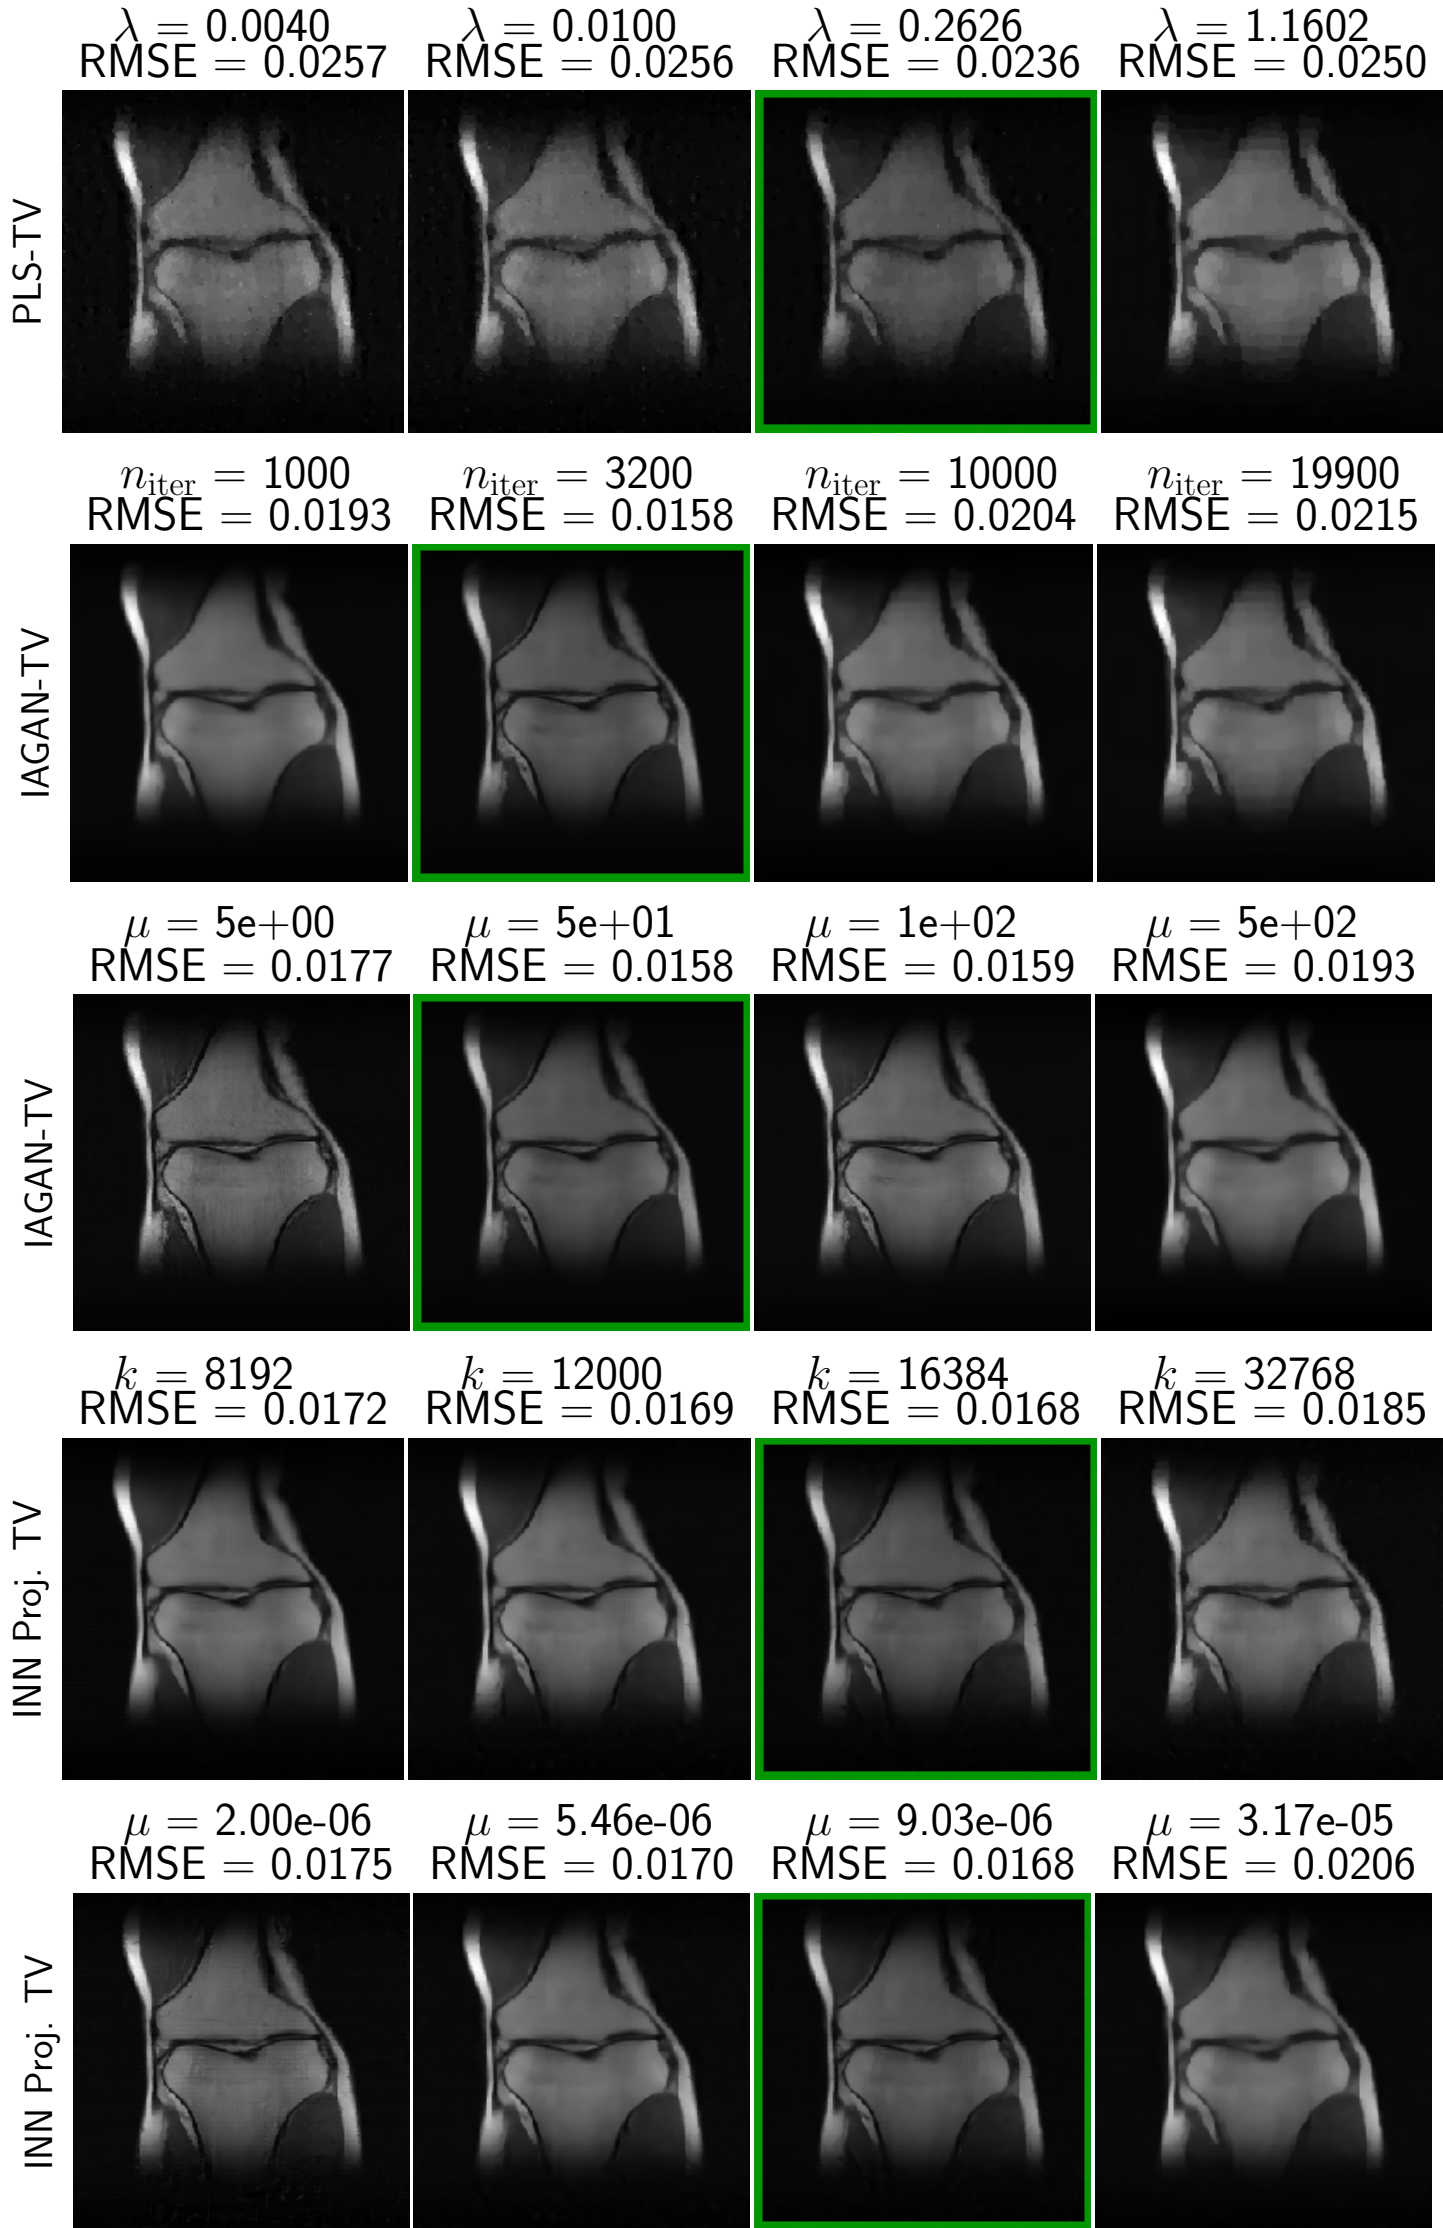    |
|              | $n_{\text{iter}} = 1000$<br>RMSE = 0.0193                                           | $n_{\text{iter}} = 3200$<br>RMSE = 0.0158                                           | $n_{\text{iter}} = 10000$<br>RMSE = 0.0204                                           | $n_{\text{iter}} = 19900$<br>RMSE = 0.0215                                            |
|              | 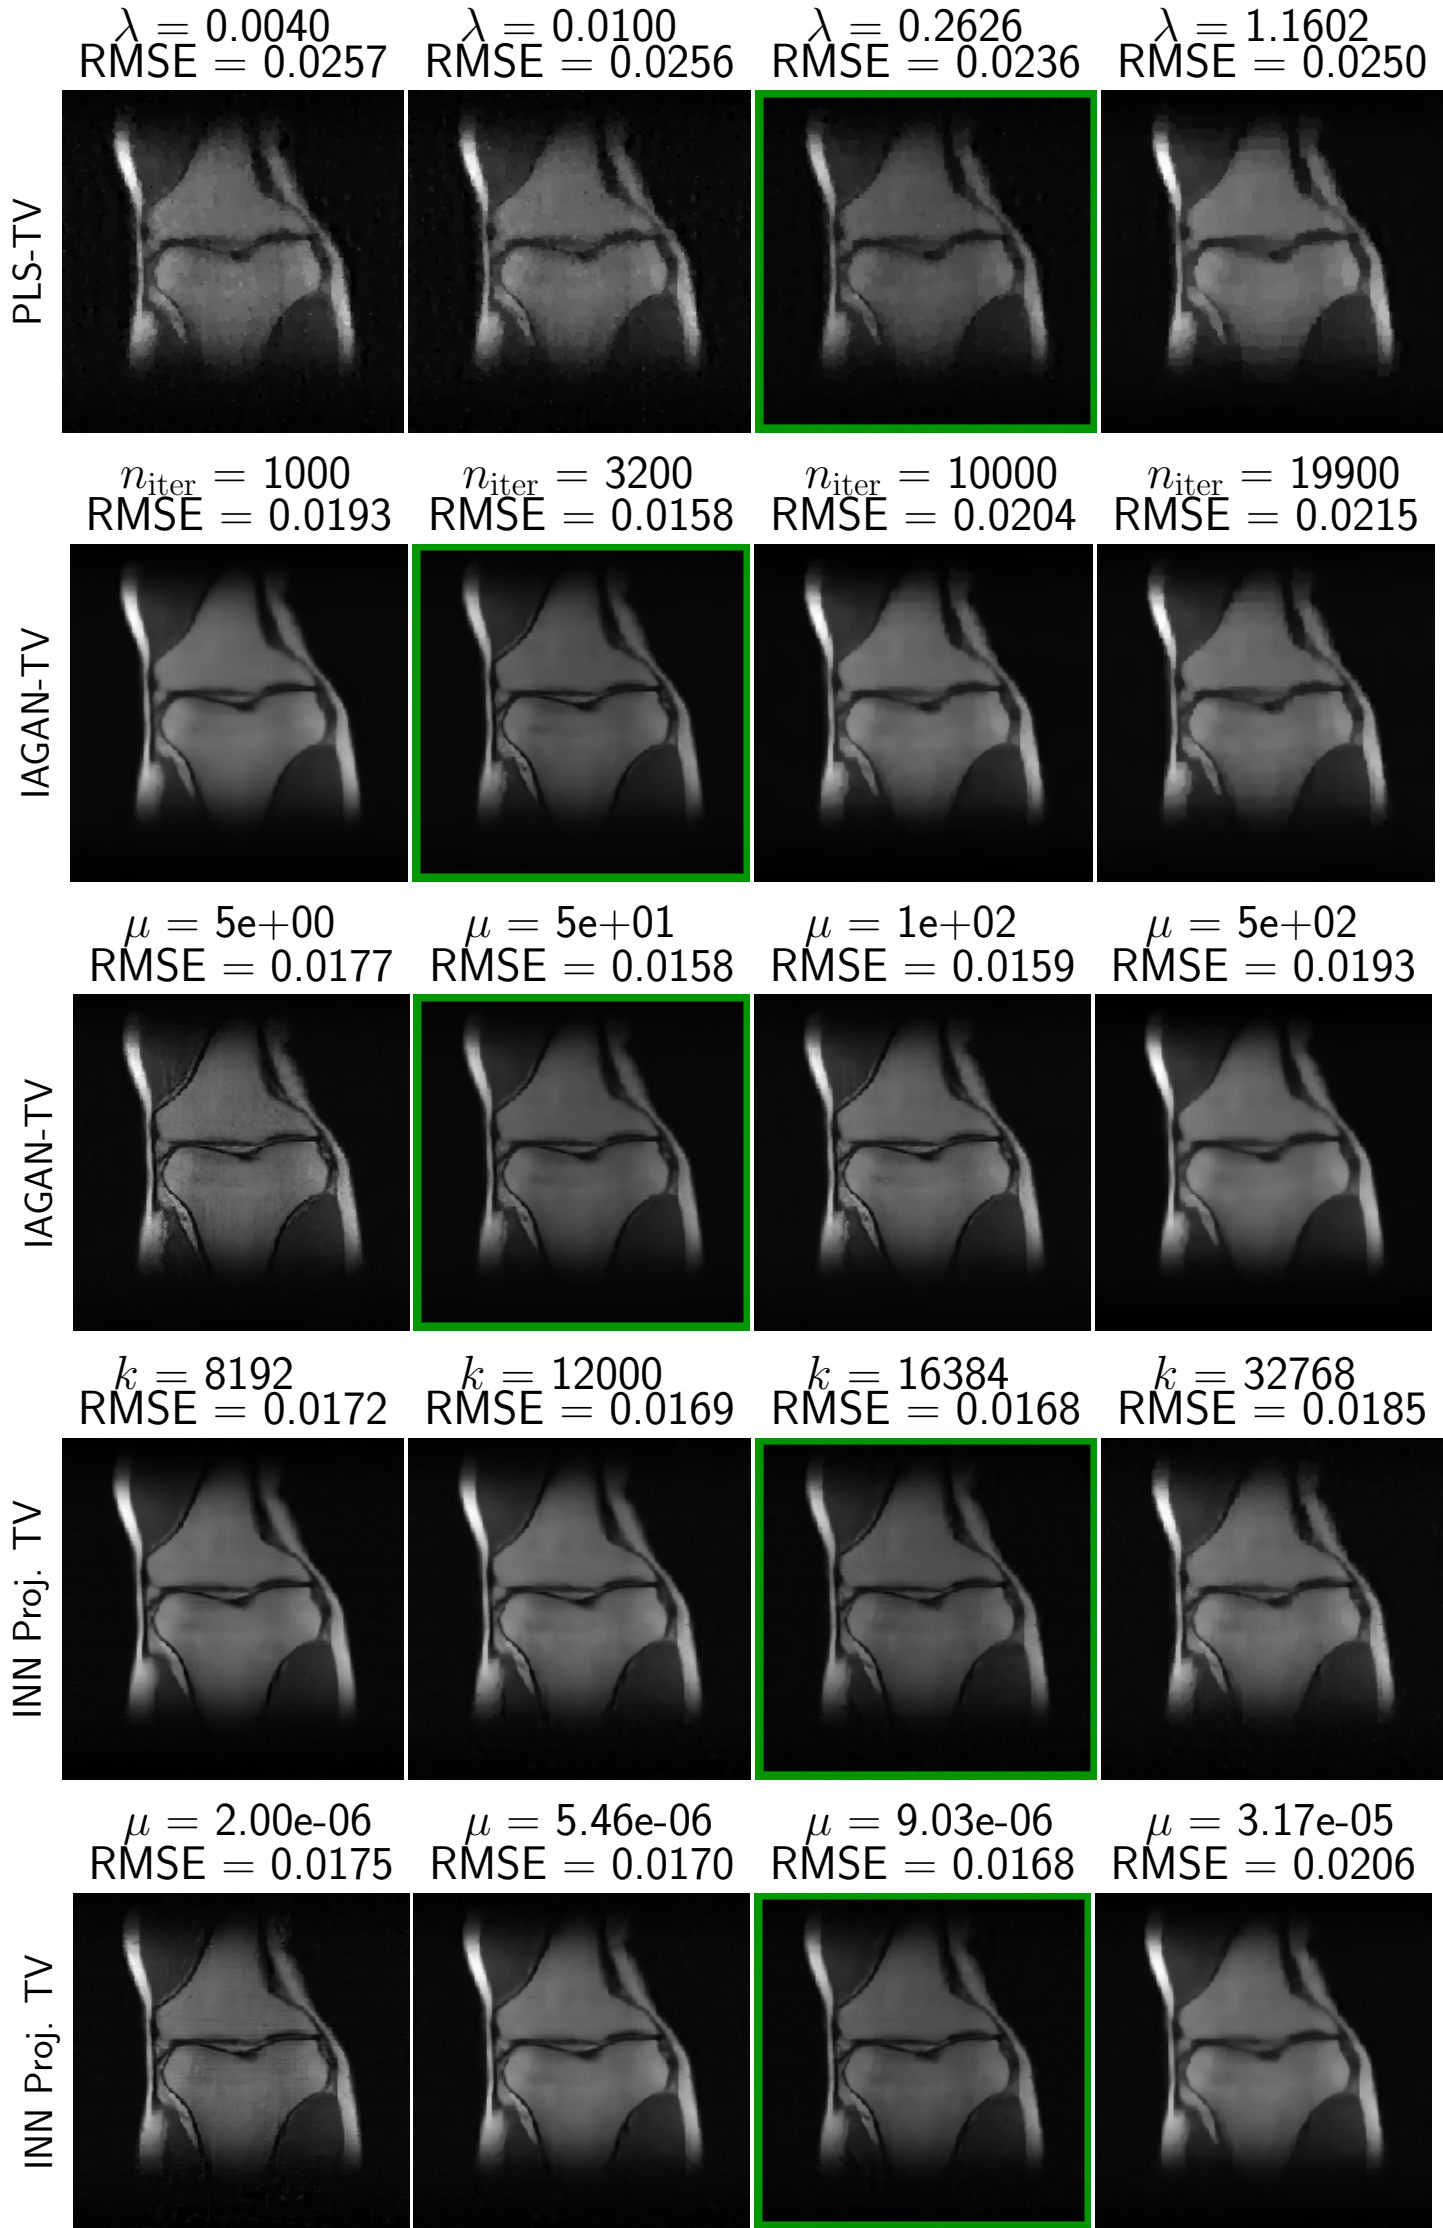   | 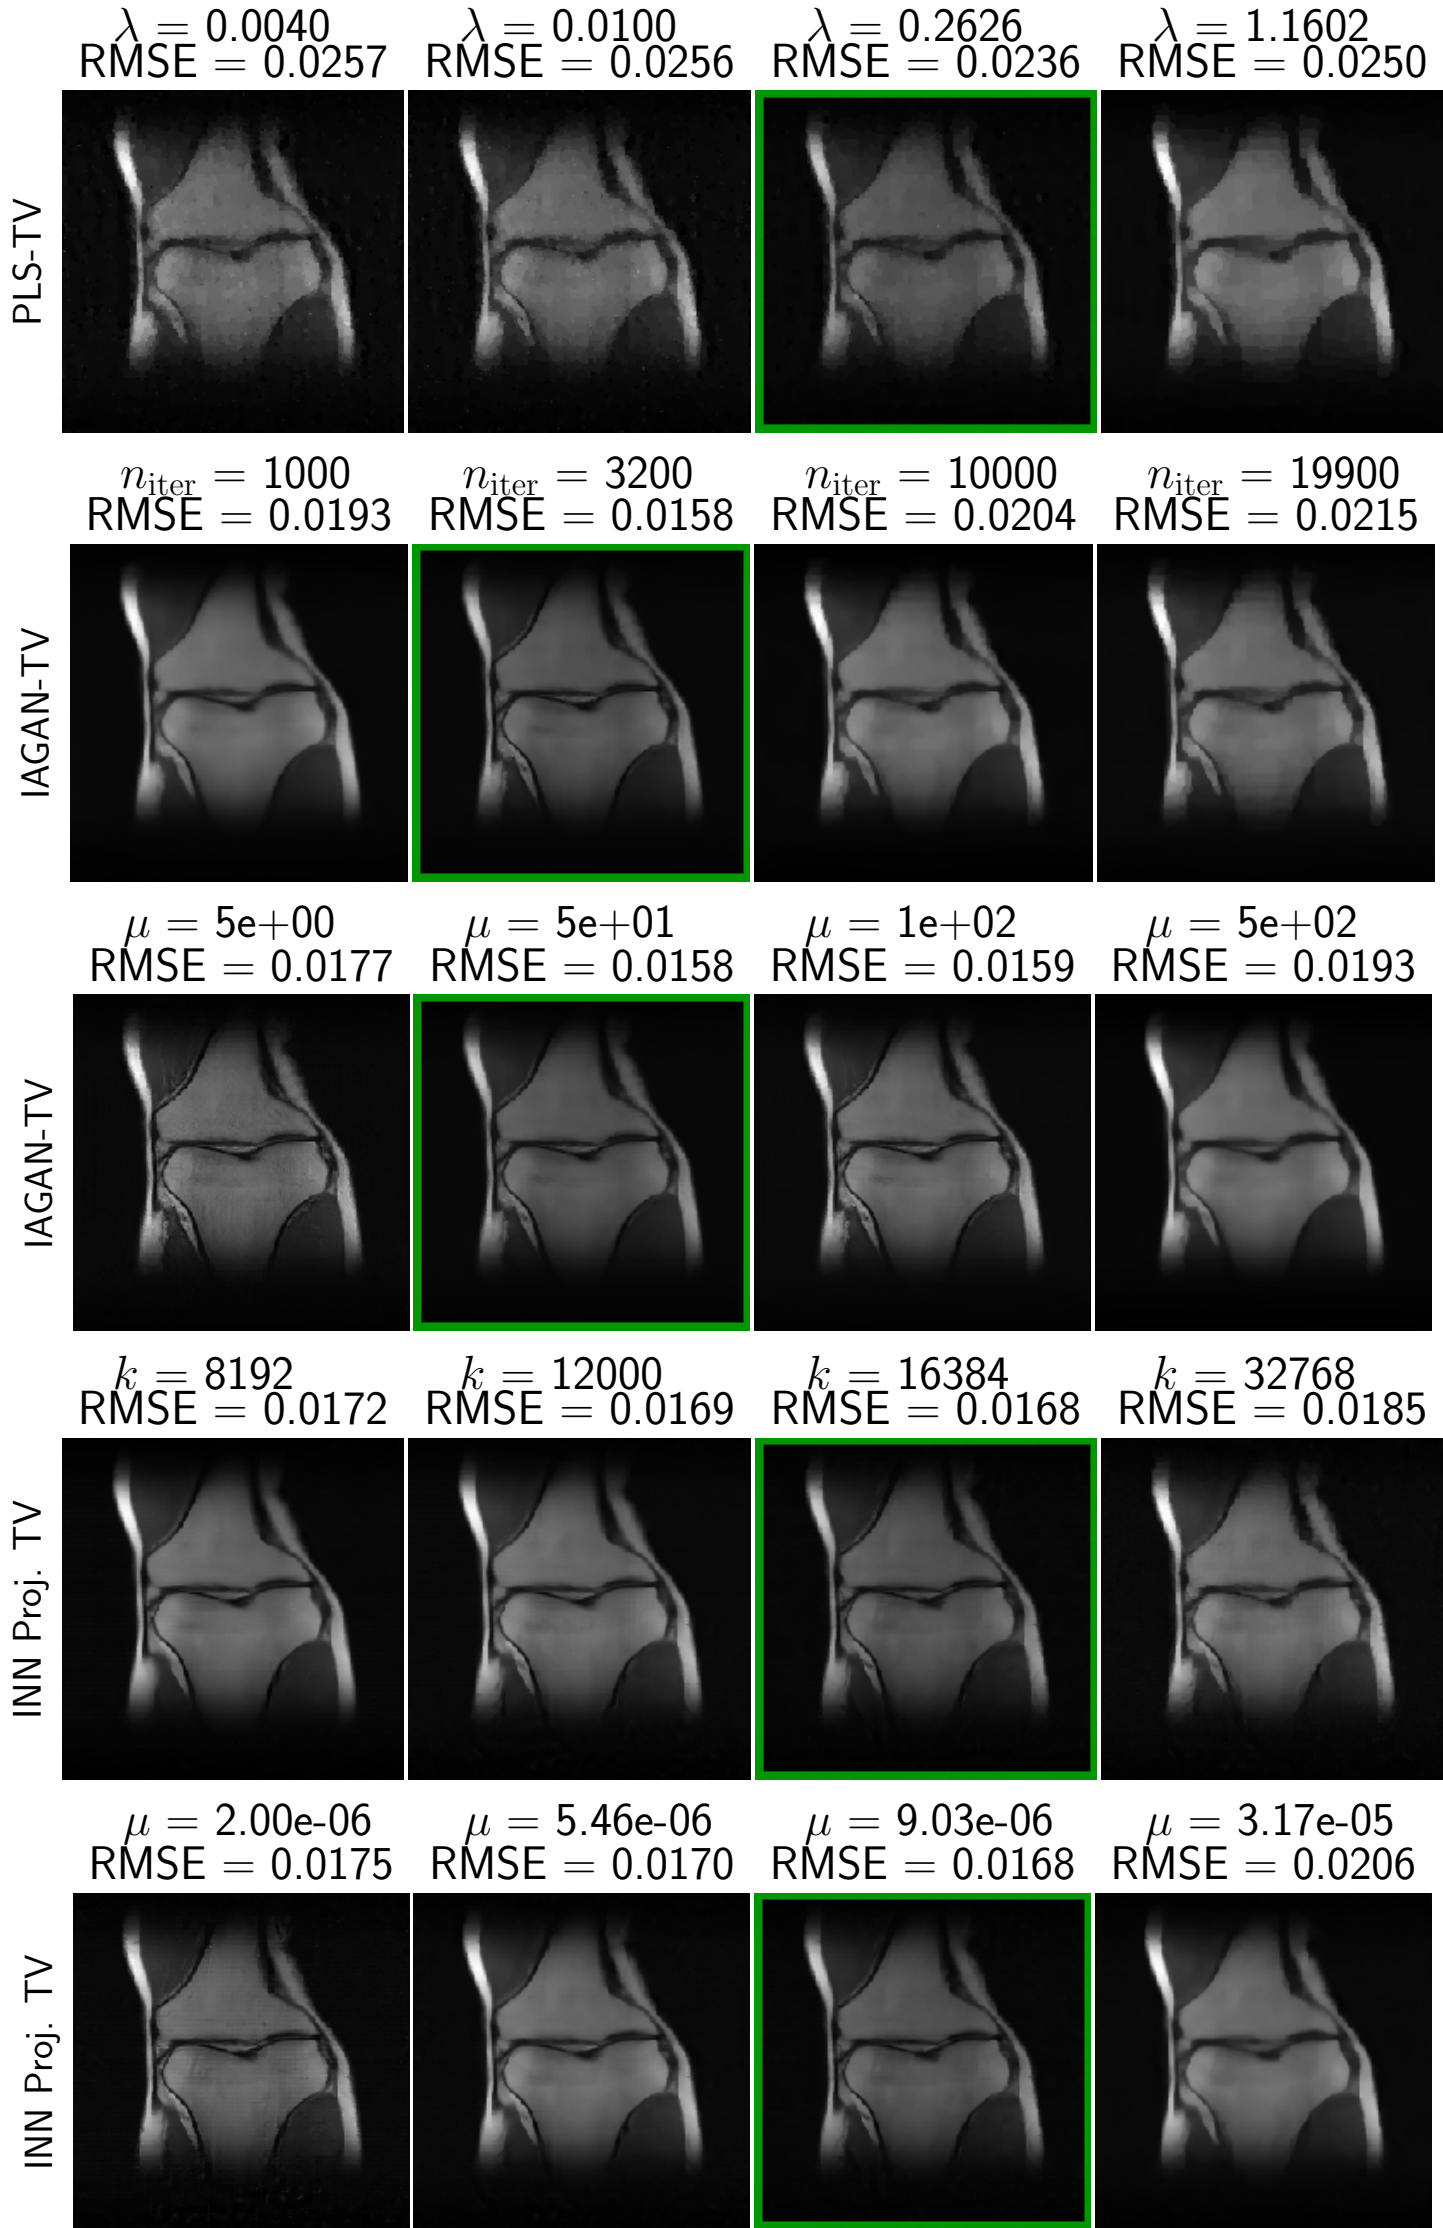   | 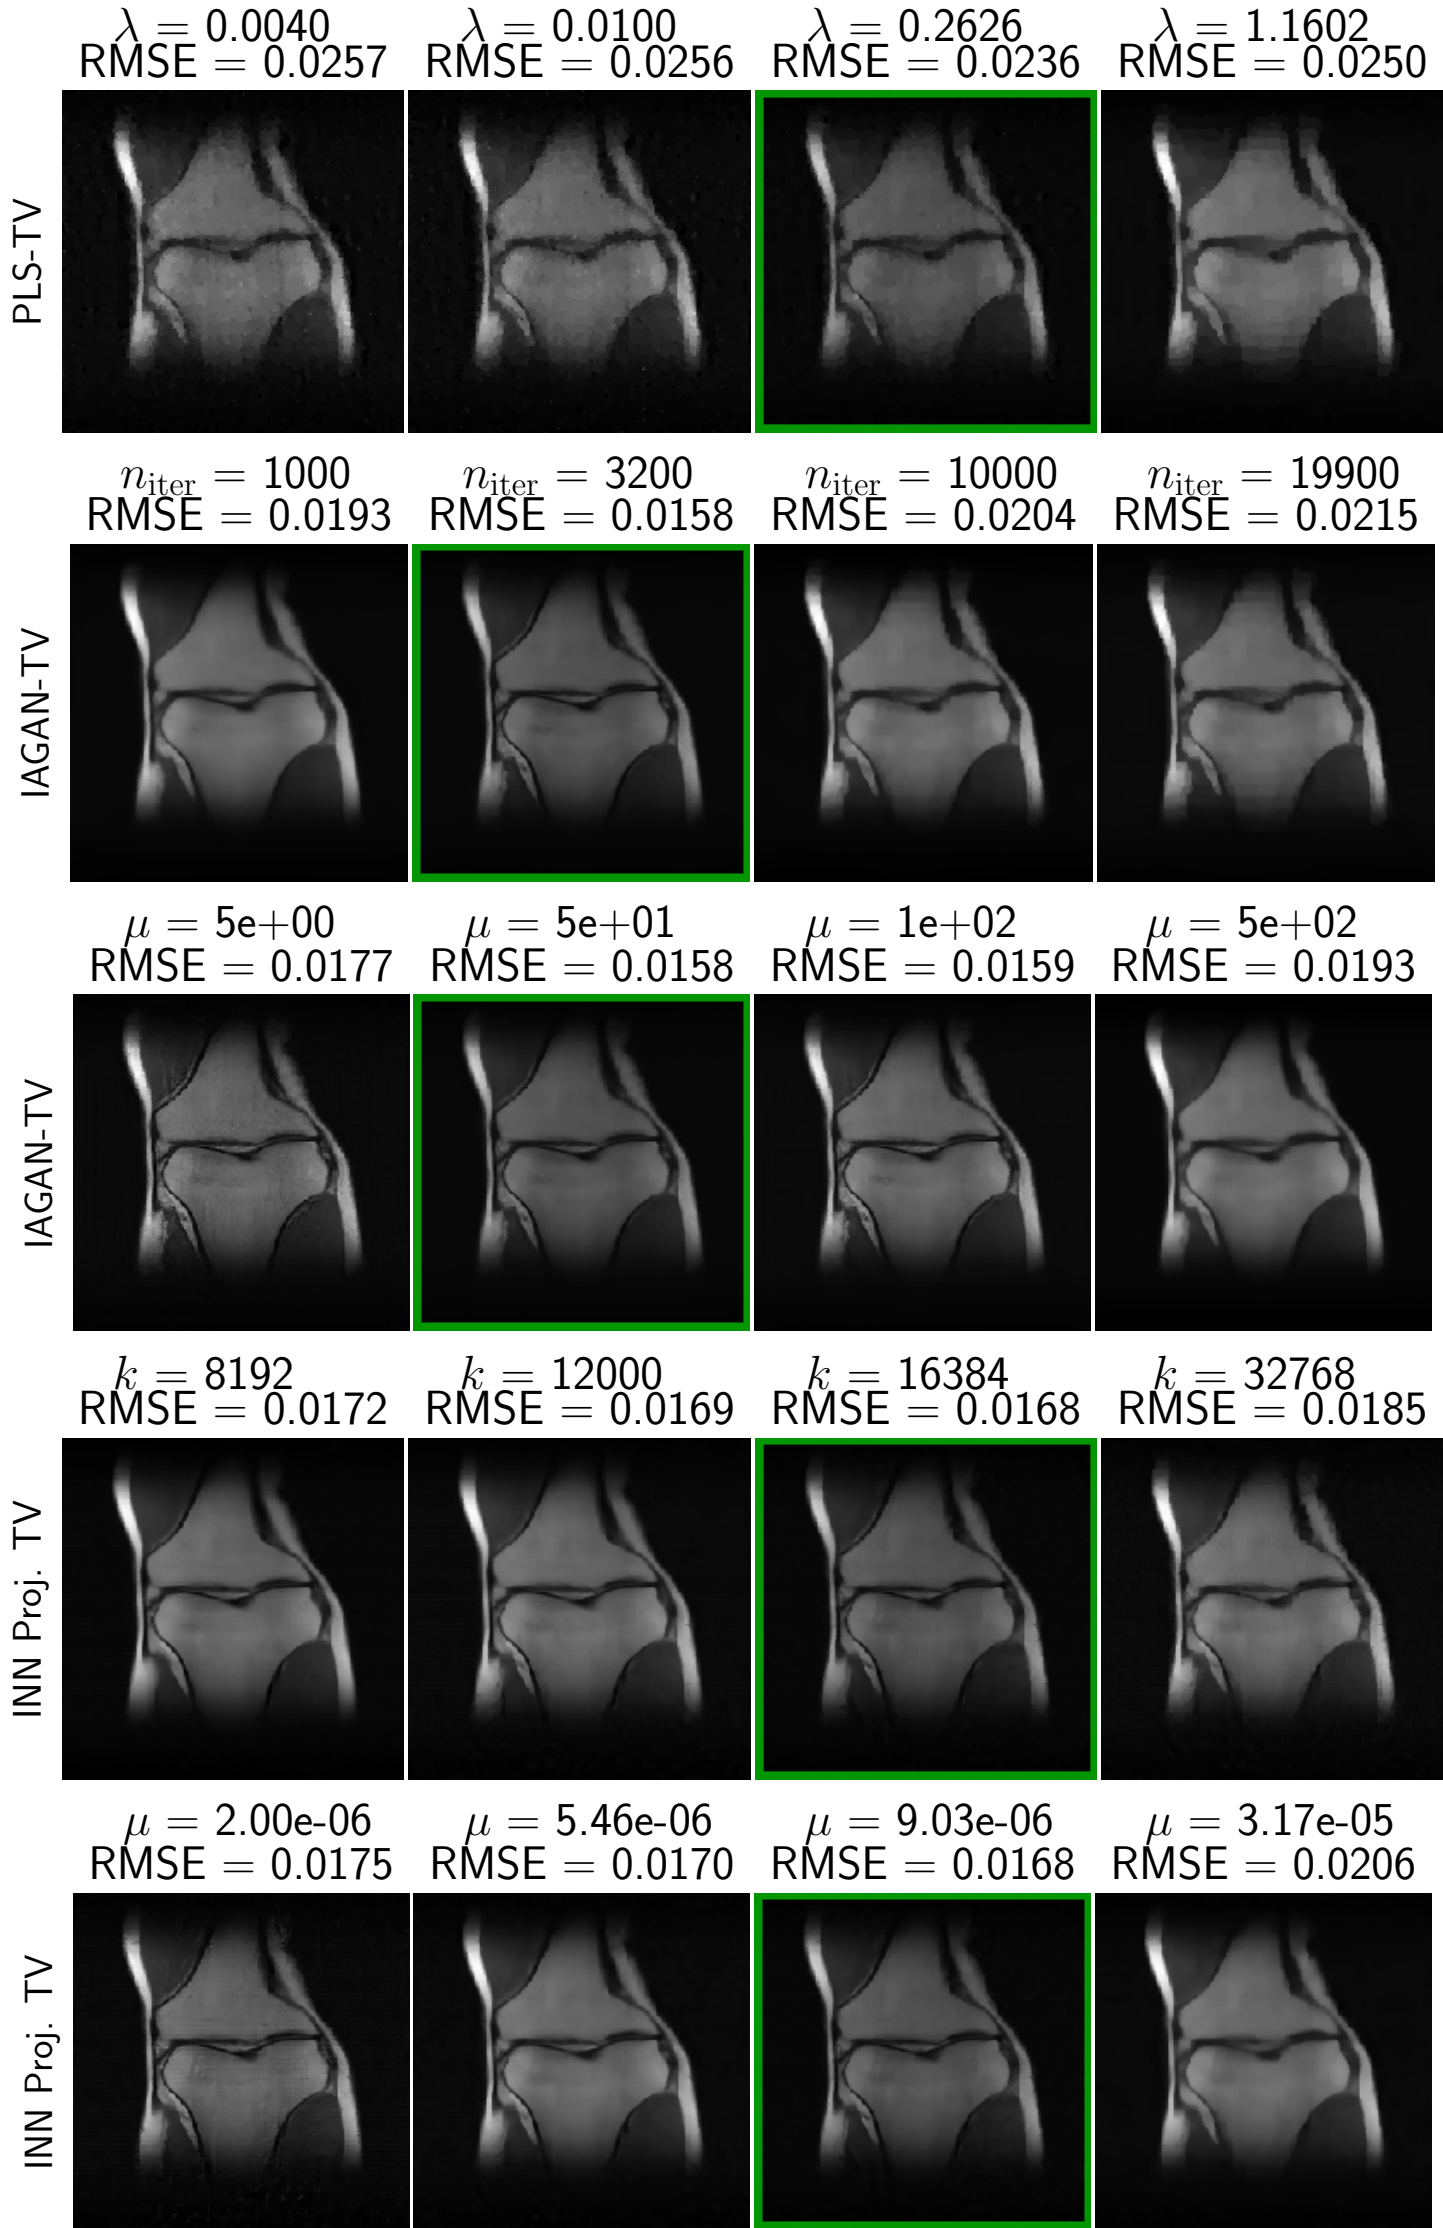   | 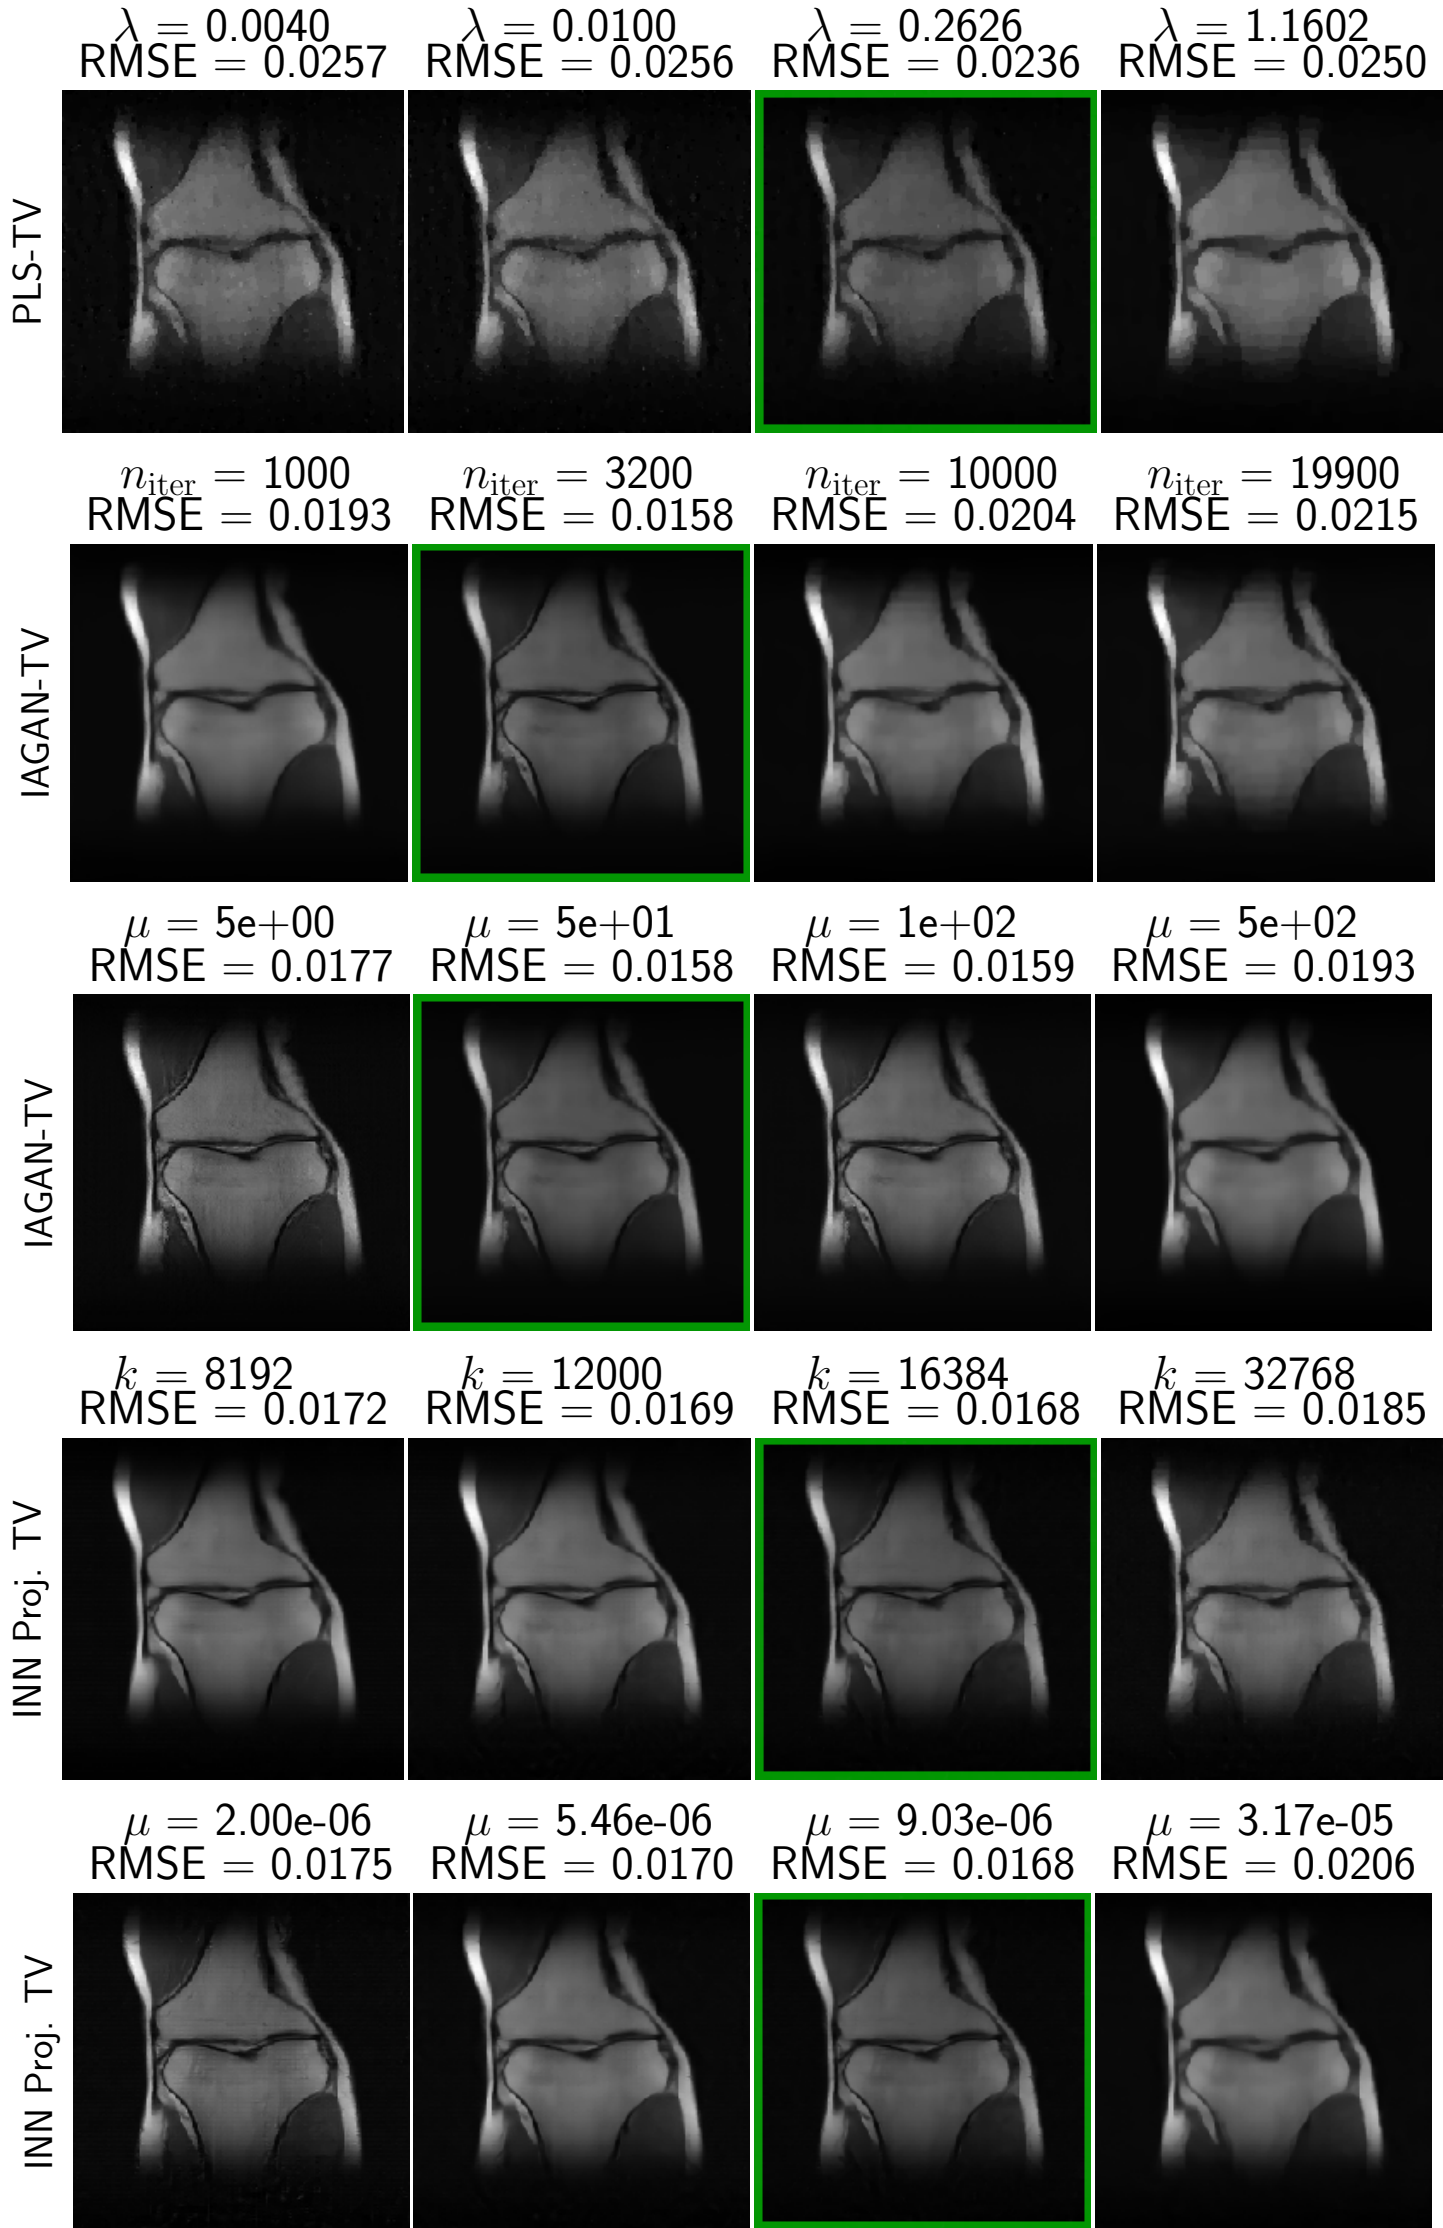   |
| IAGAN-TV     | $\mu = 5e+00$<br>RMSE = 0.0177                                                      | $\mu = 5e+01$<br>RMSE = 0.0158                                                      | $\mu = 1e+02$<br>RMSE = 0.0159                                                       | $\mu = 5e+02$<br>RMSE = 0.0193                                                        |
|              | 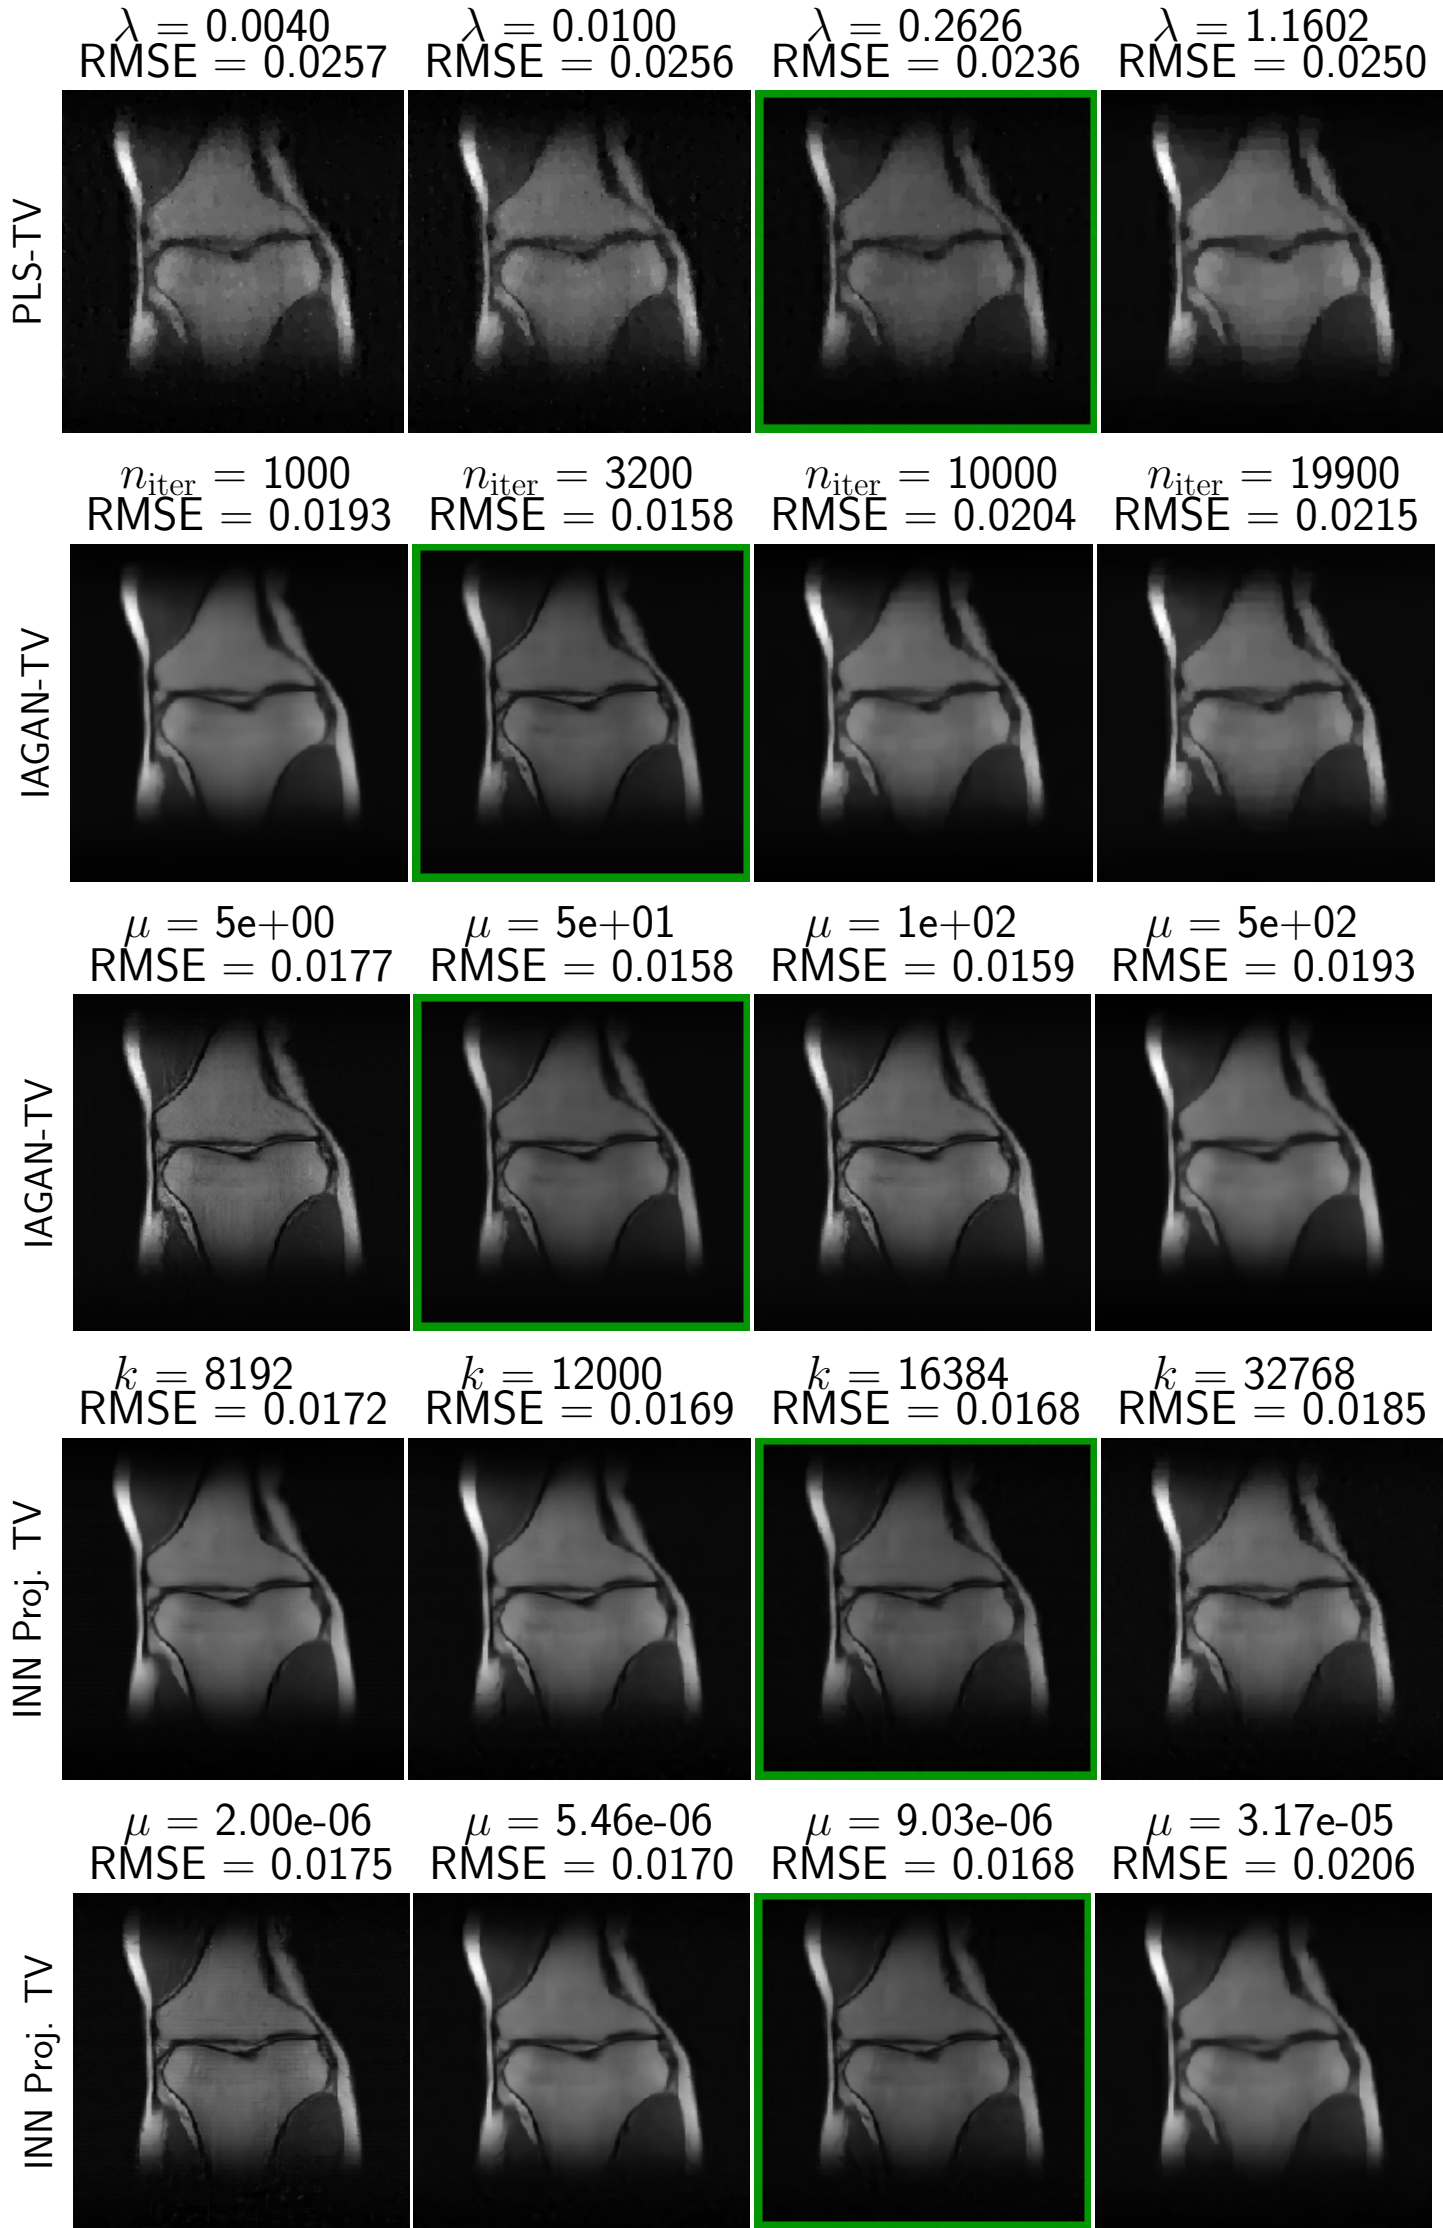  | 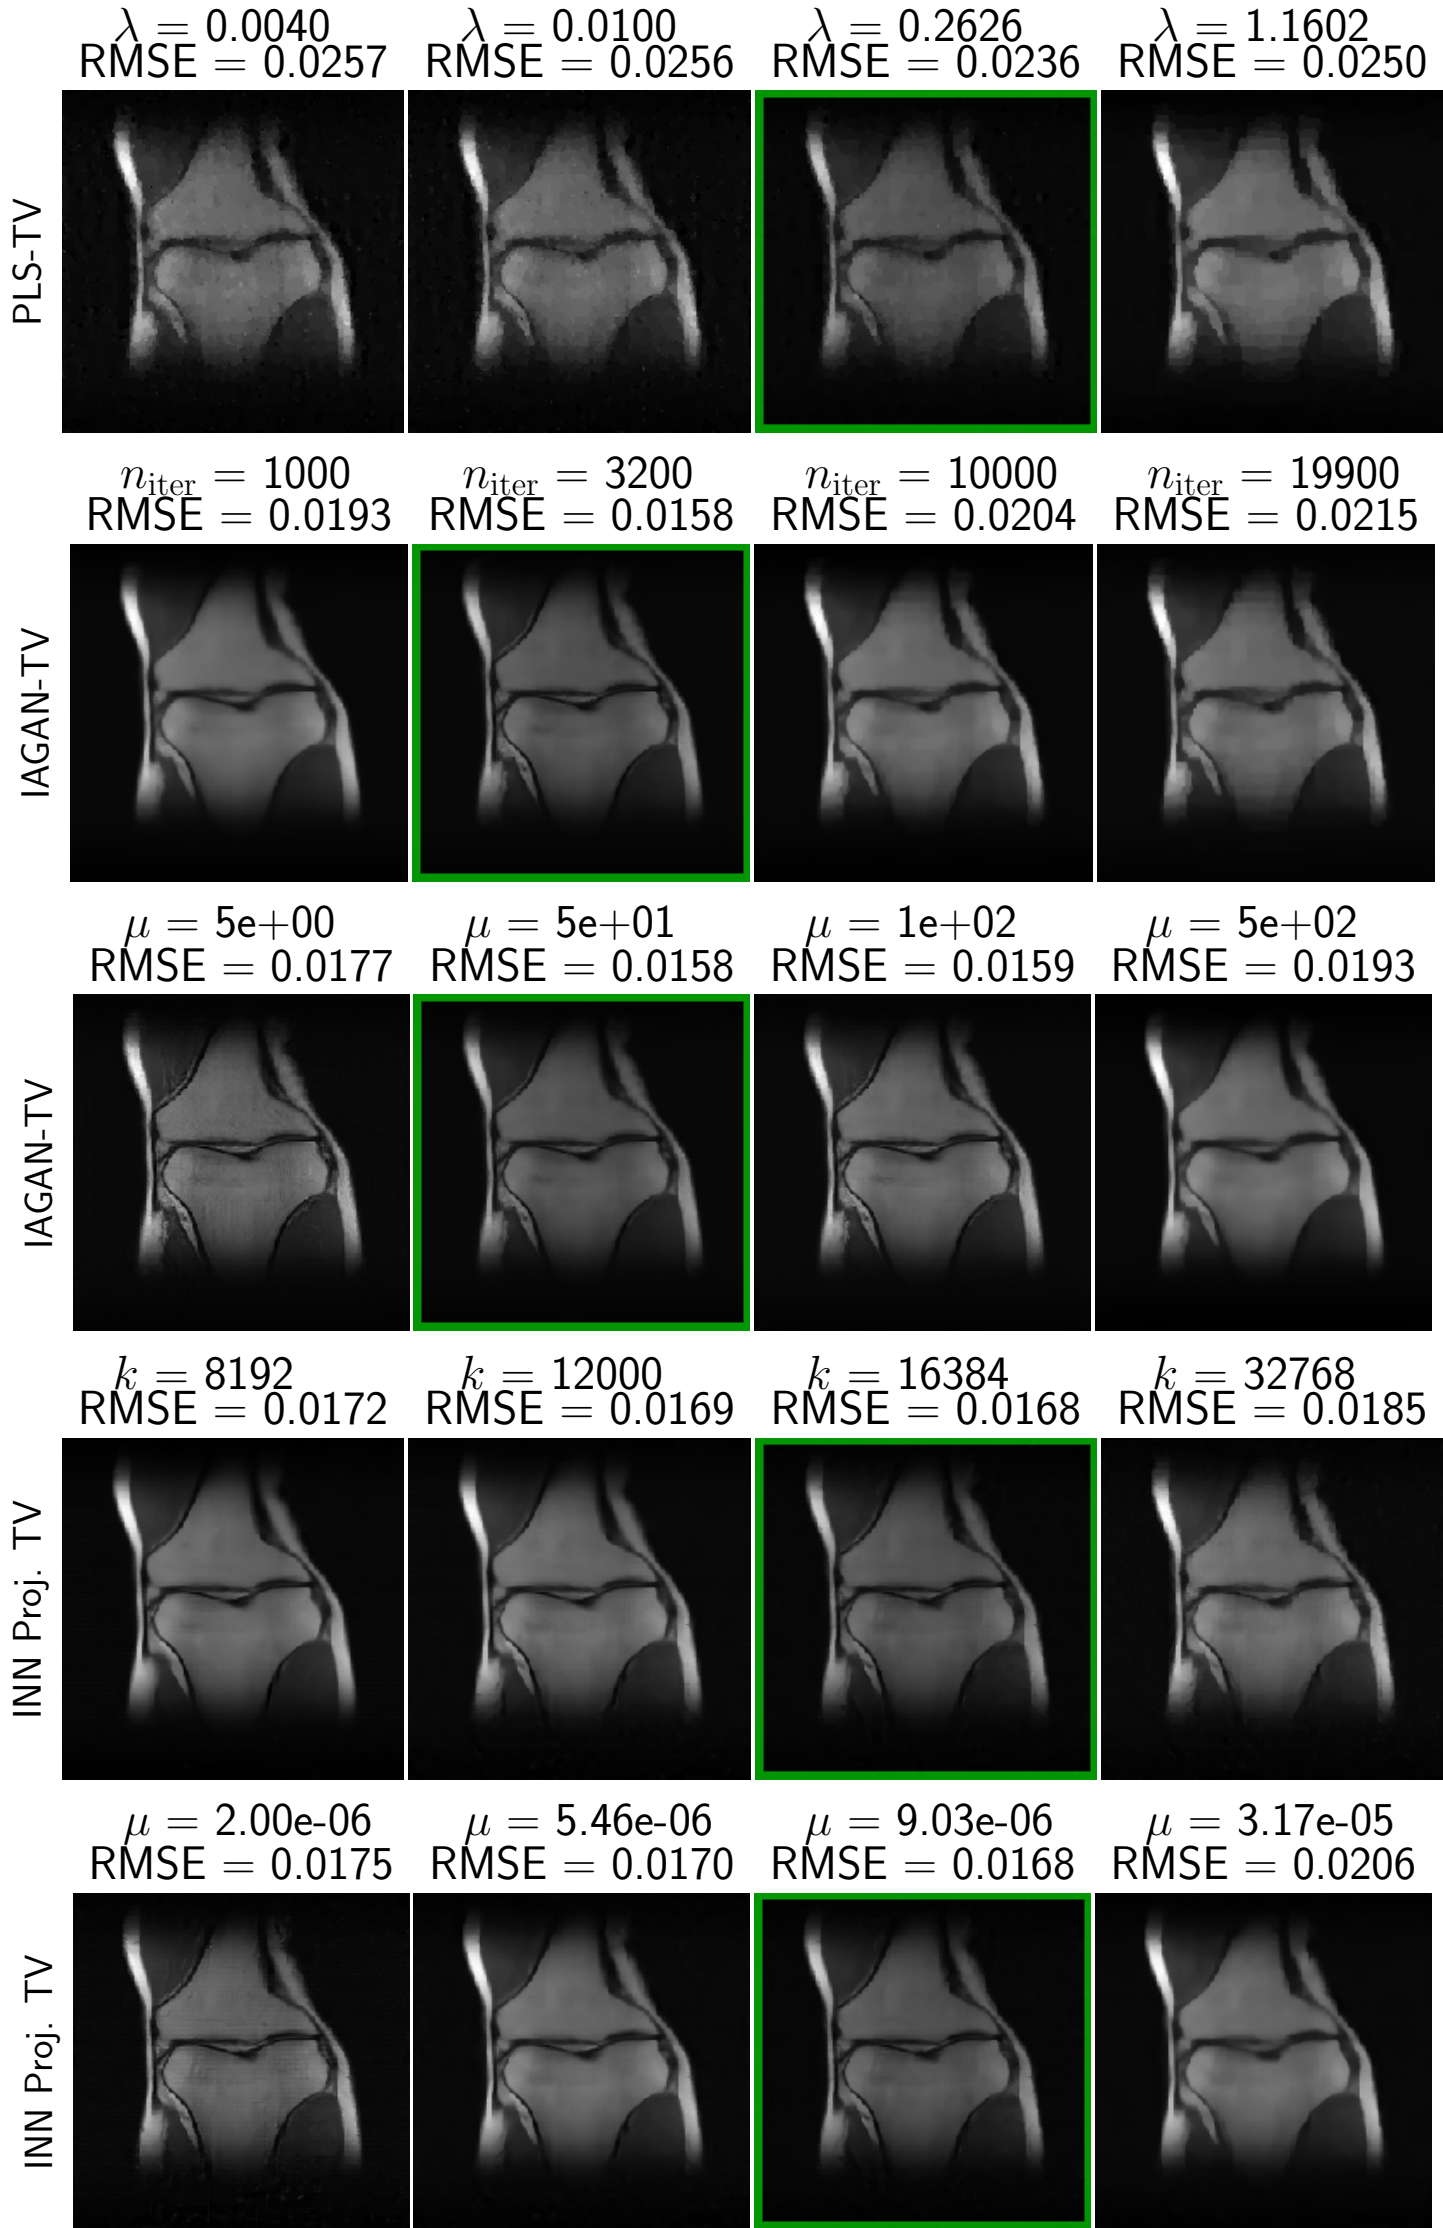  | 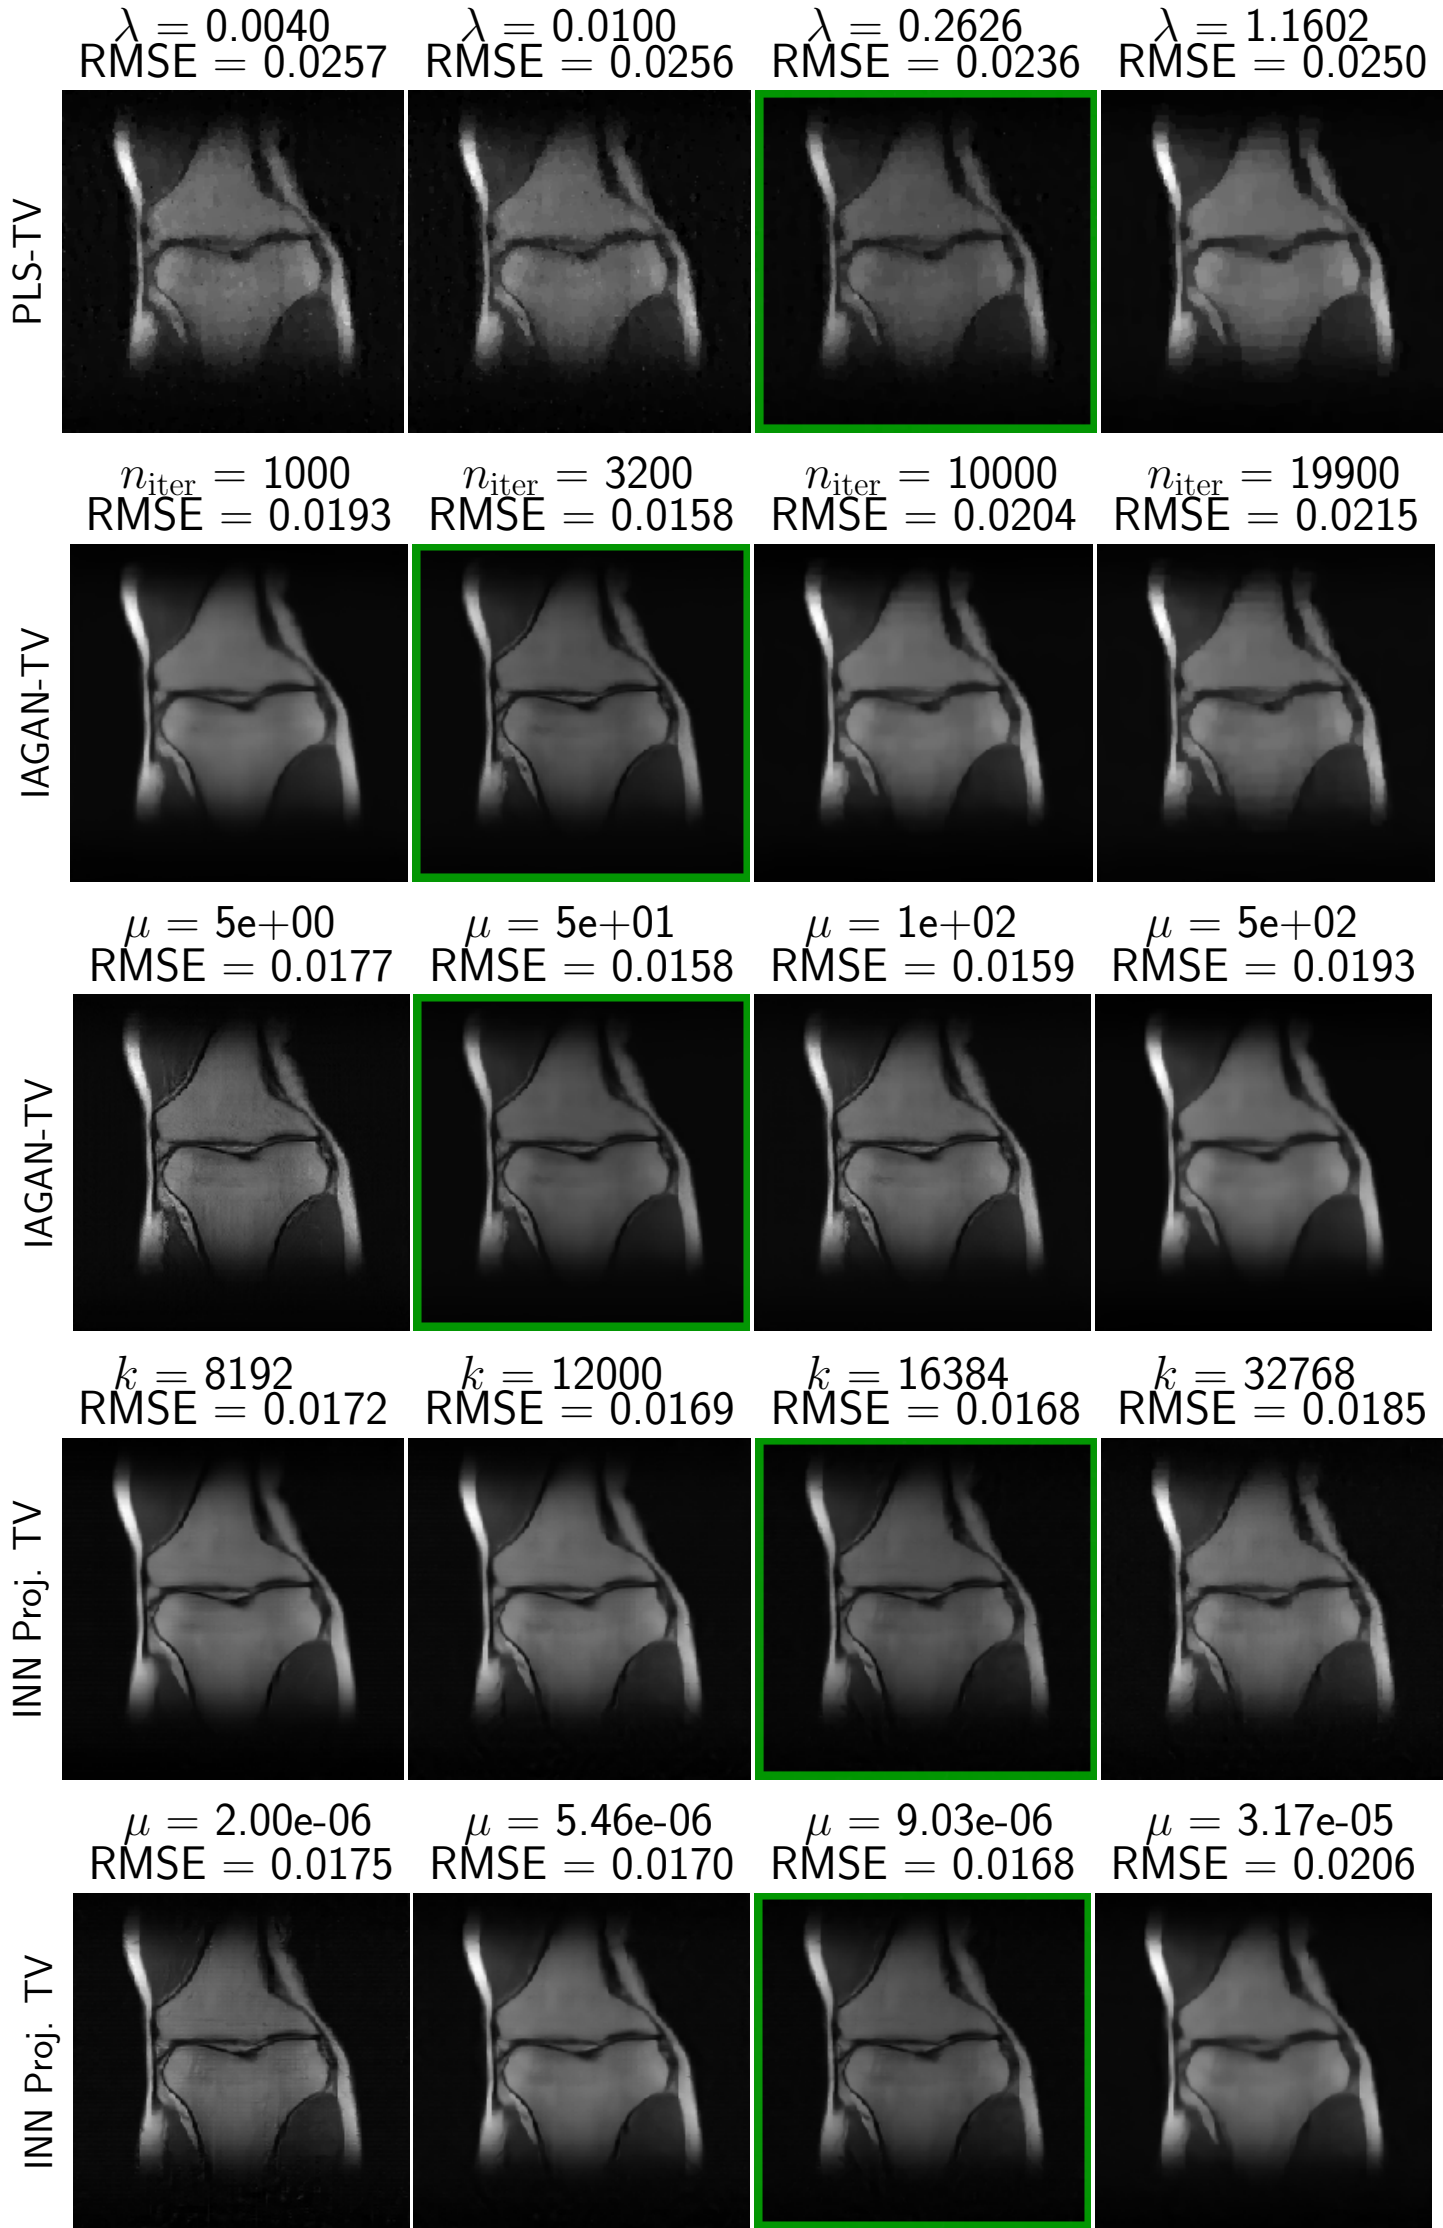  | 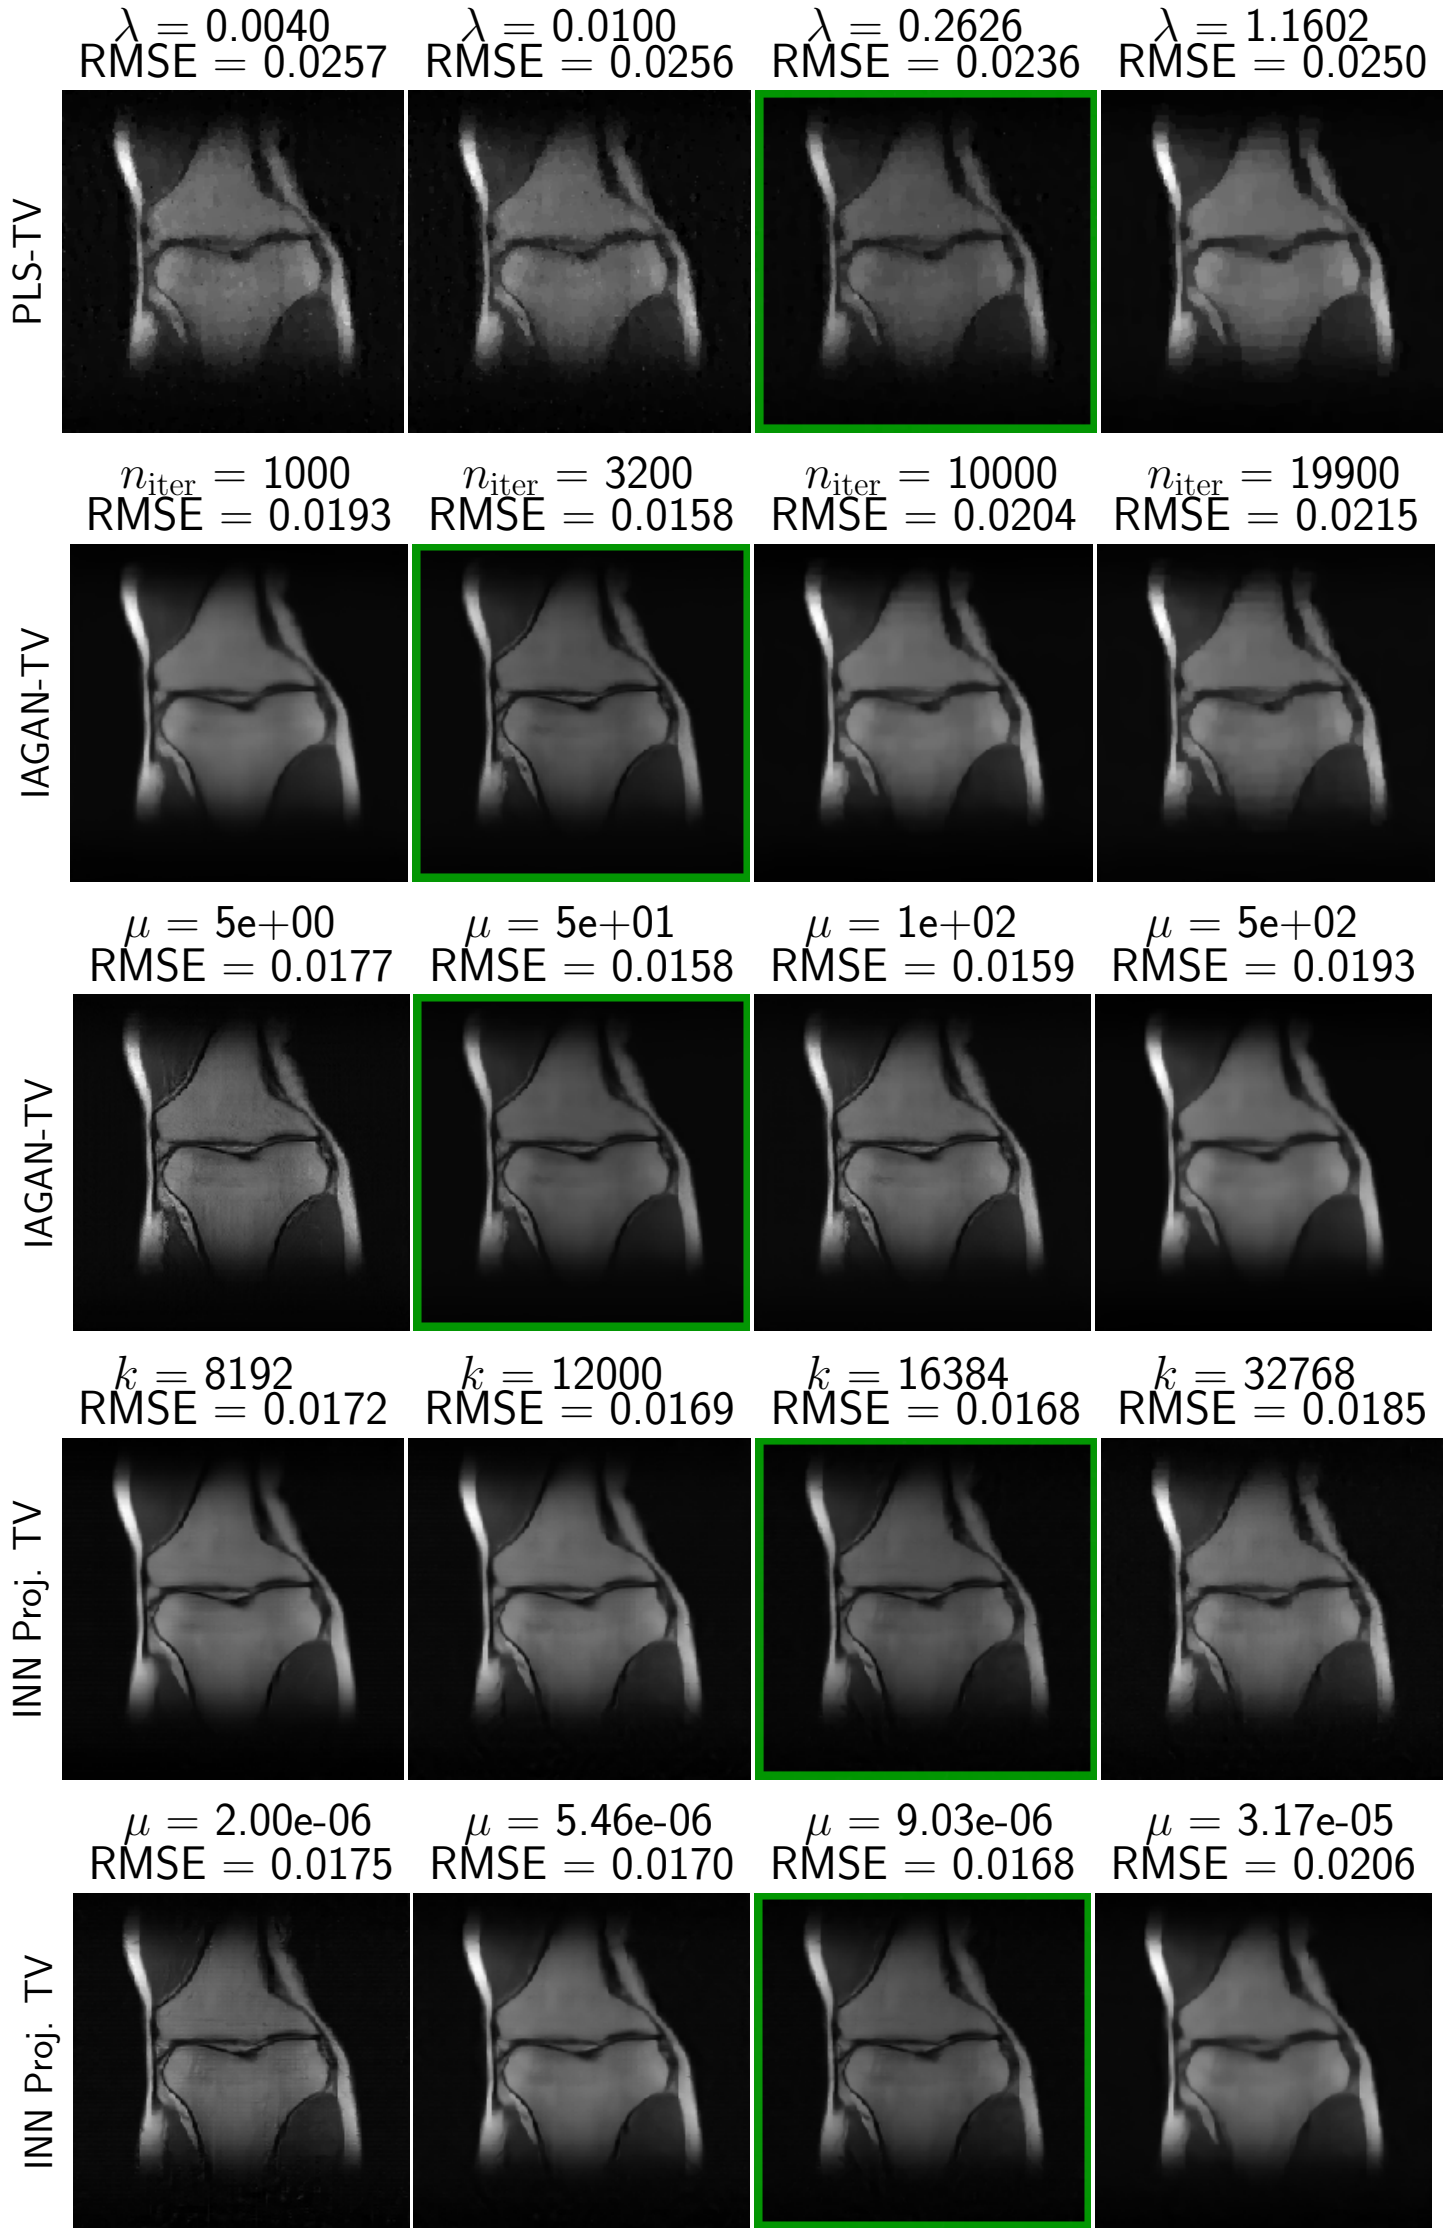  |
|              | $k = 8192$<br>RMSE = 0.0172                                                         | $k = 12000$<br>RMSE = 0.0169                                                        | $k = 16384$<br>RMSE = 0.0168                                                         | $k = 32768$<br>RMSE = 0.0185                                                          |
|              | 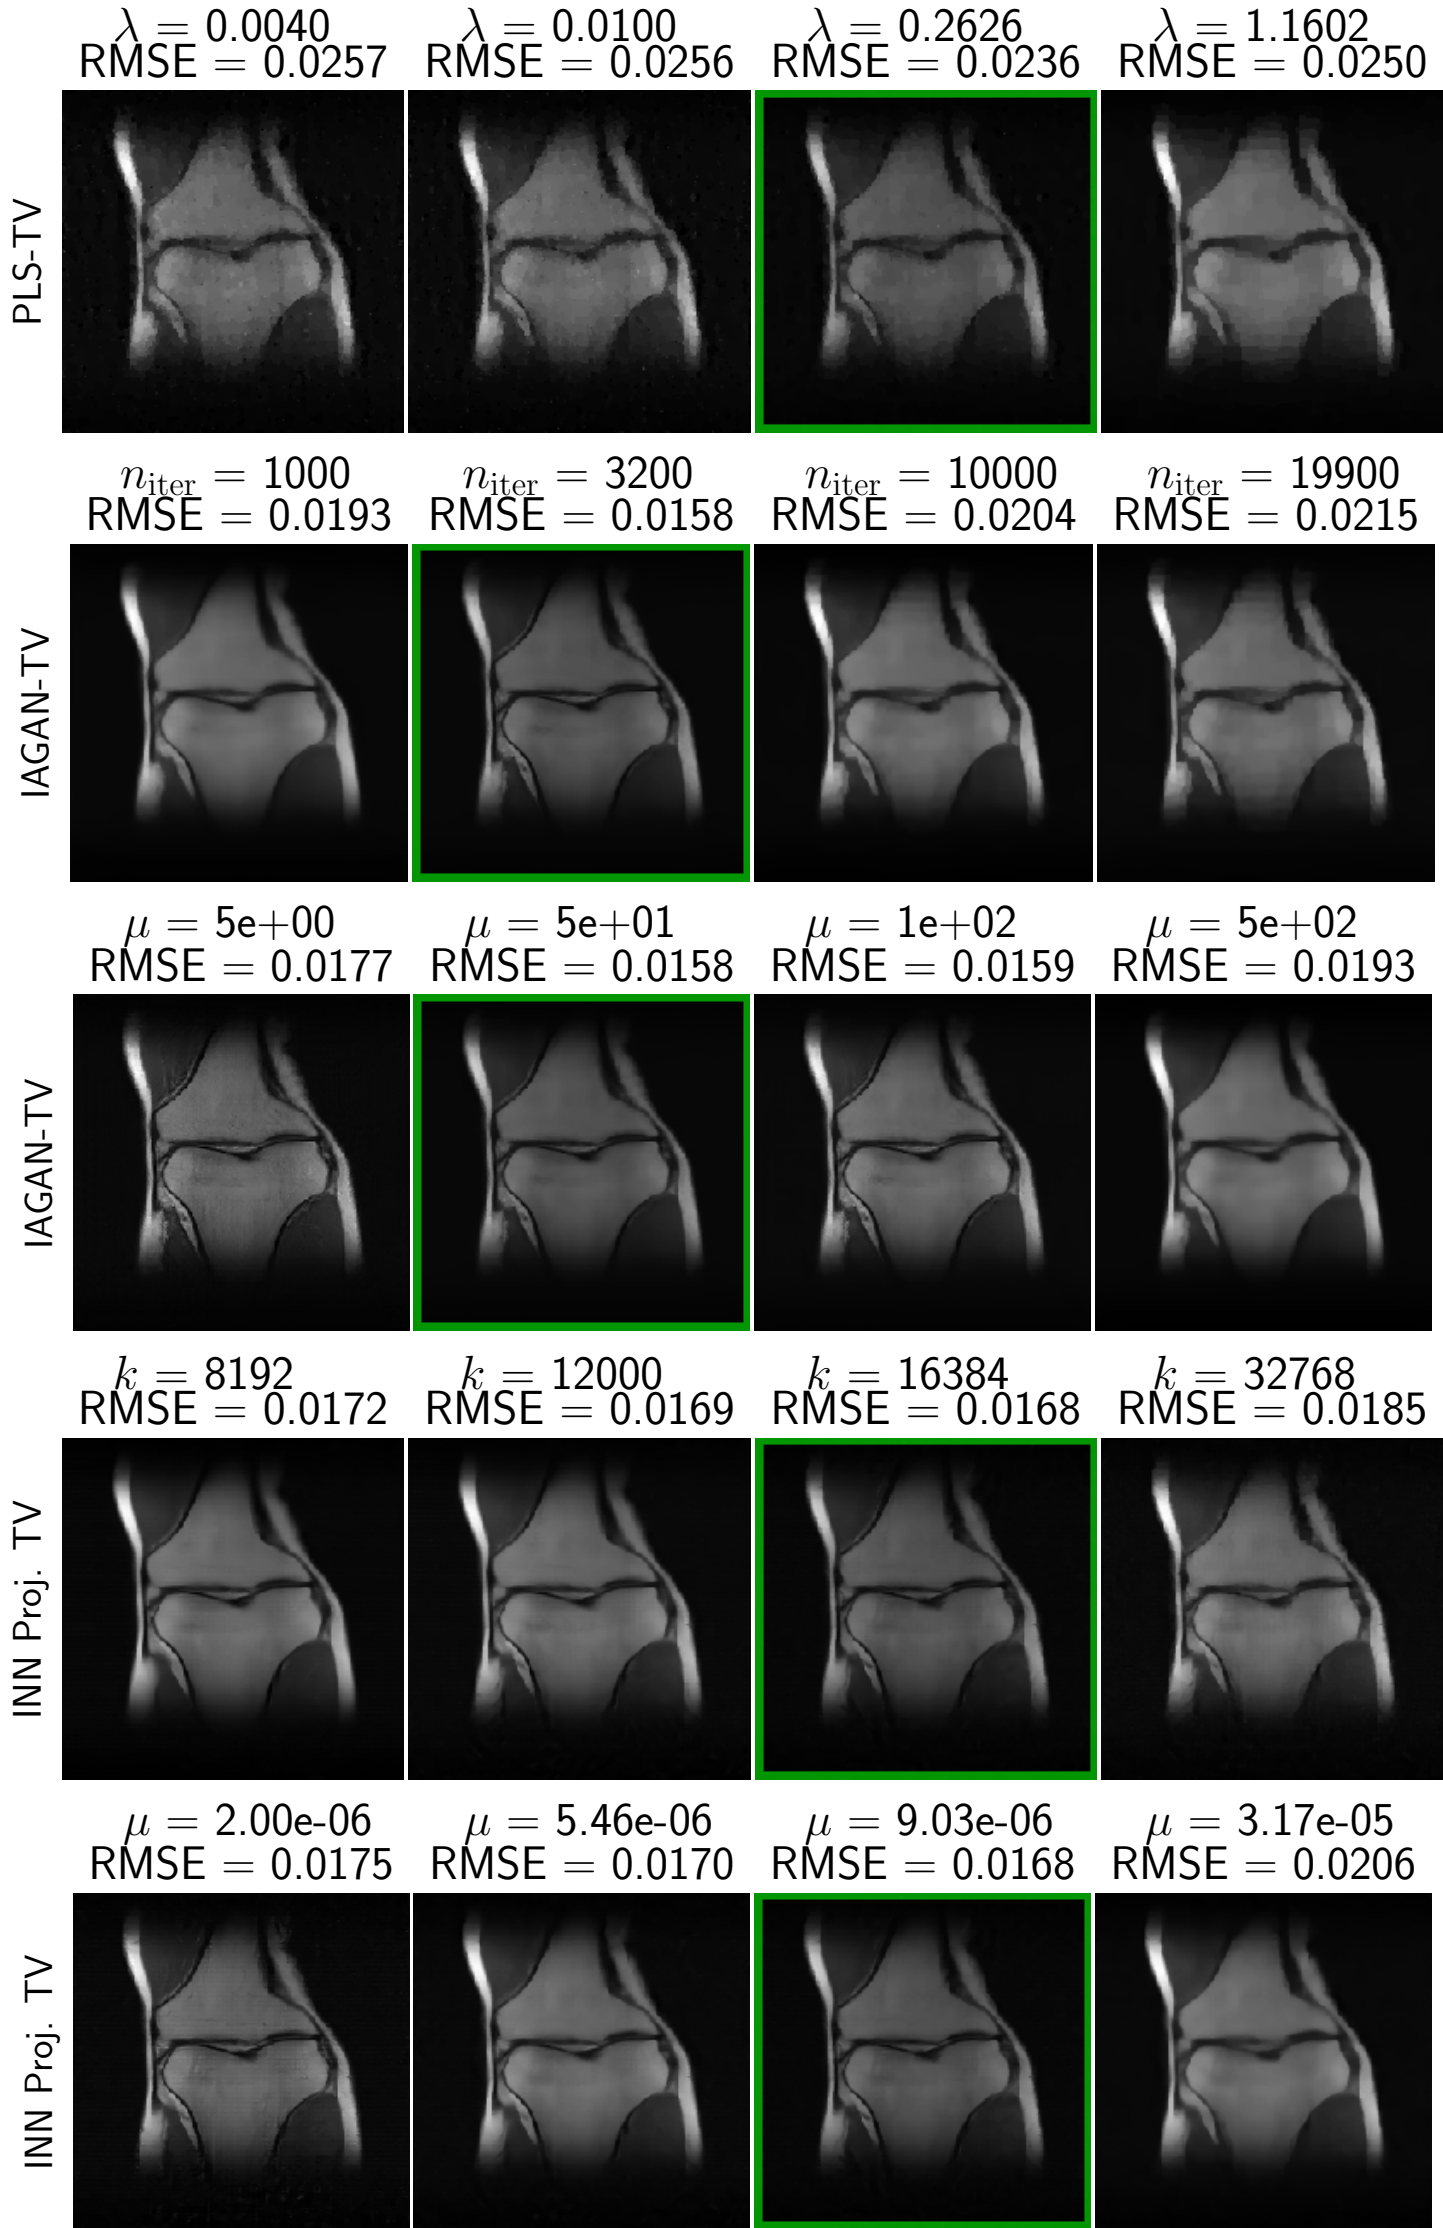 | 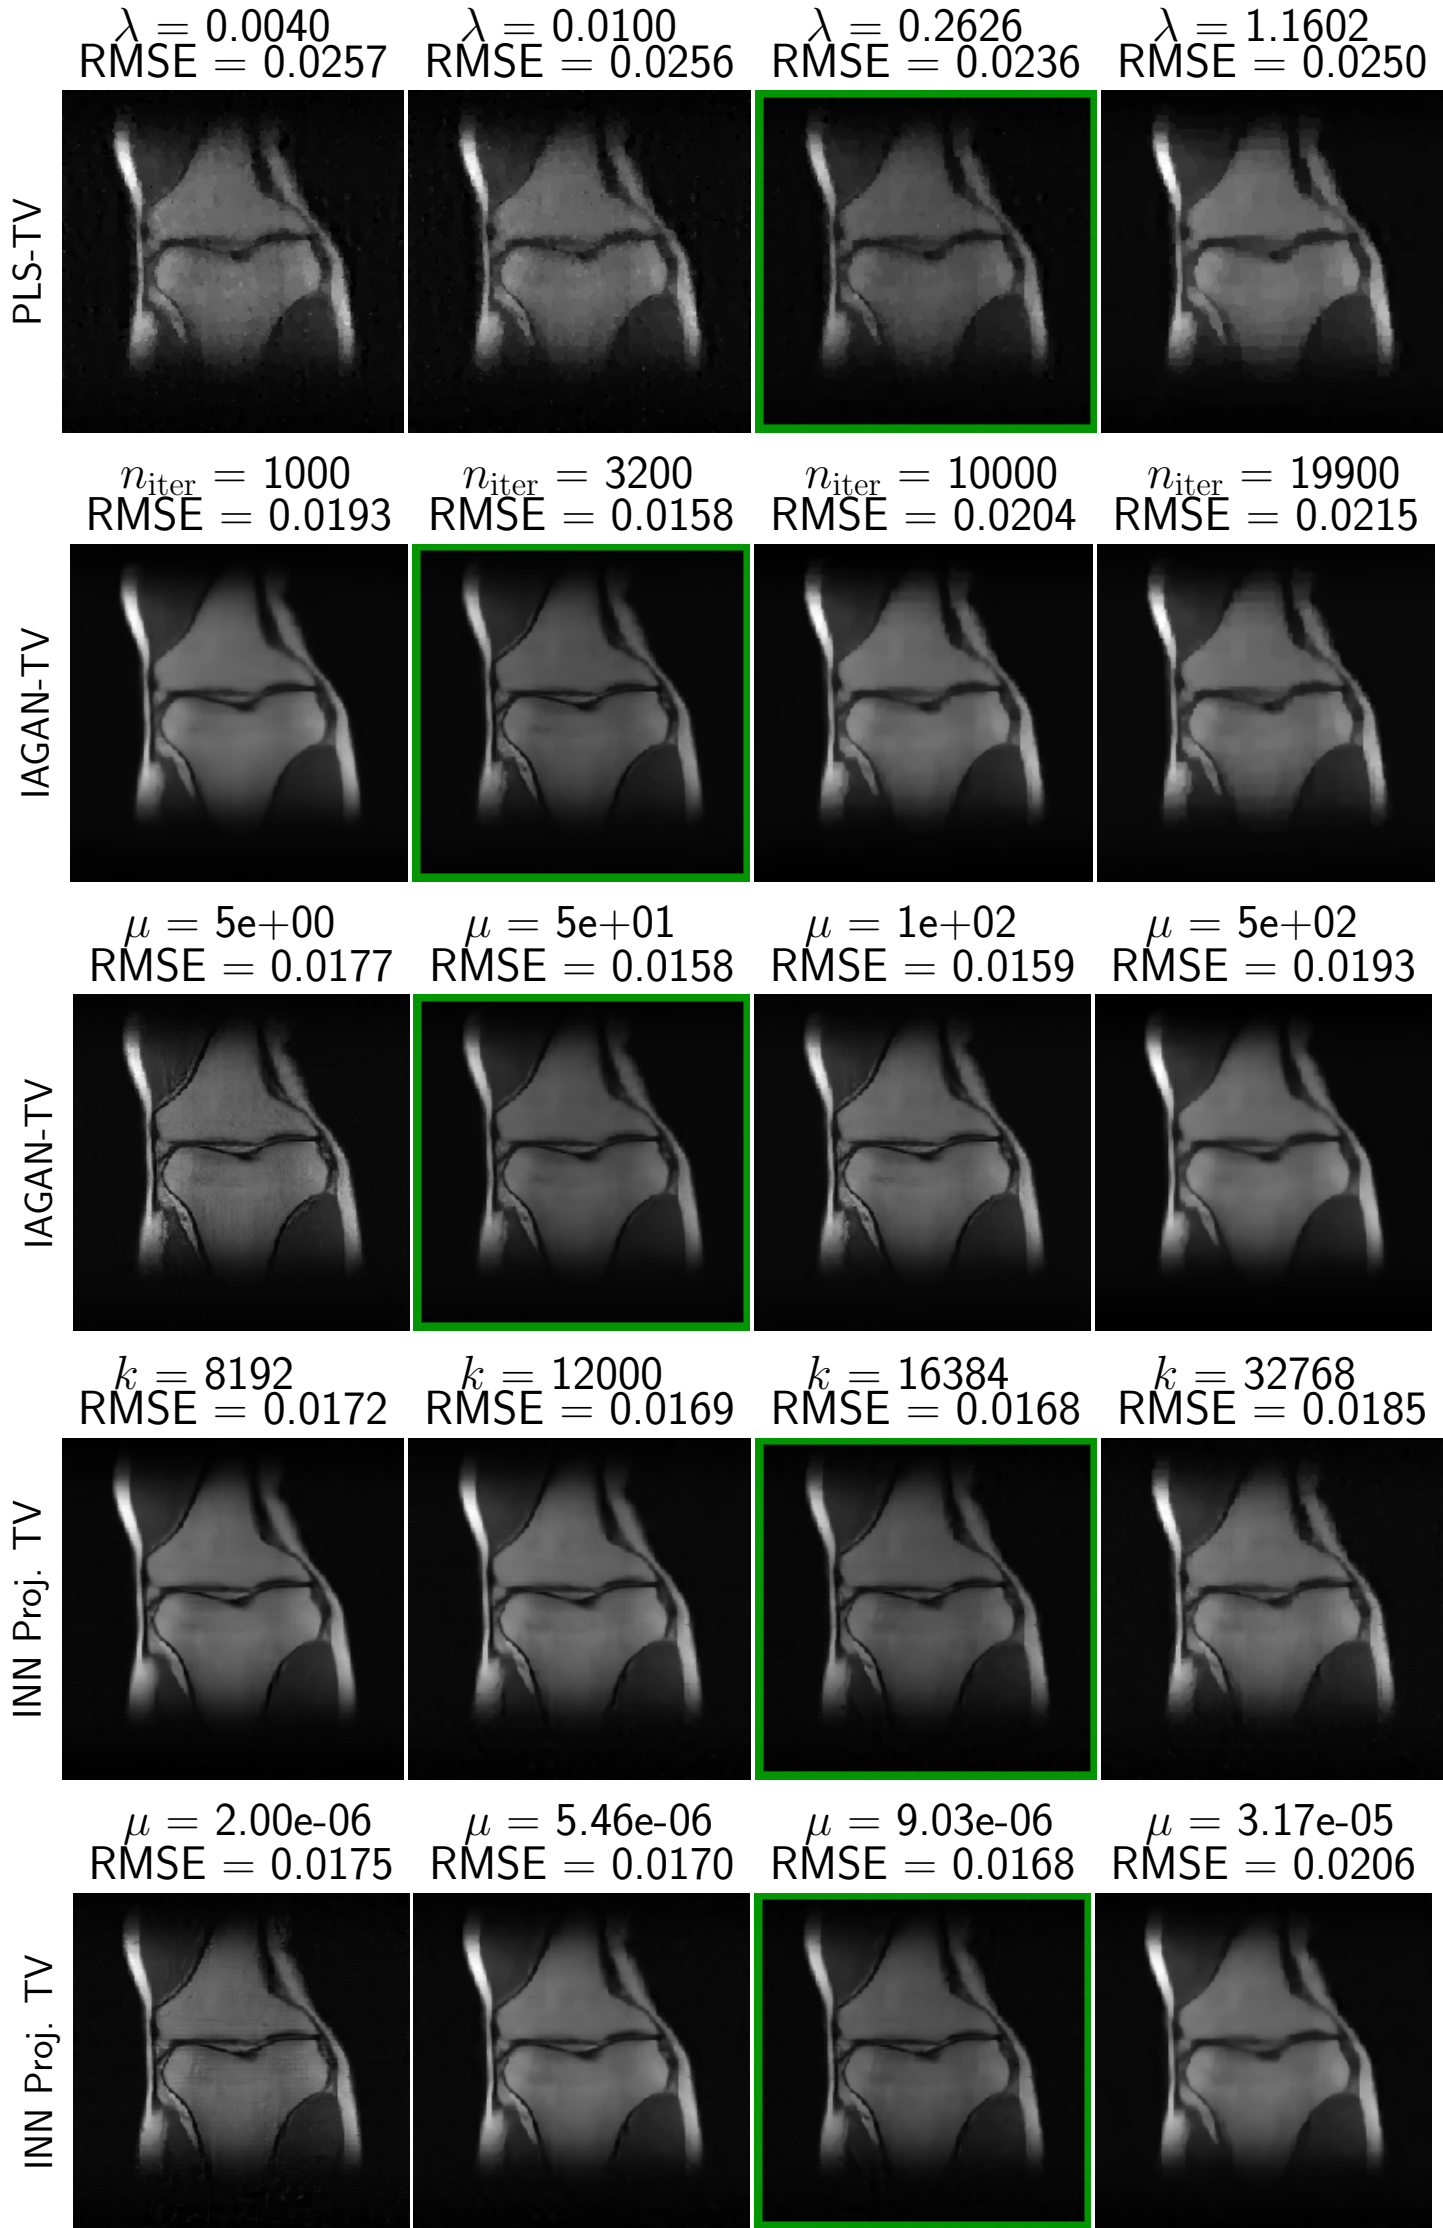 | 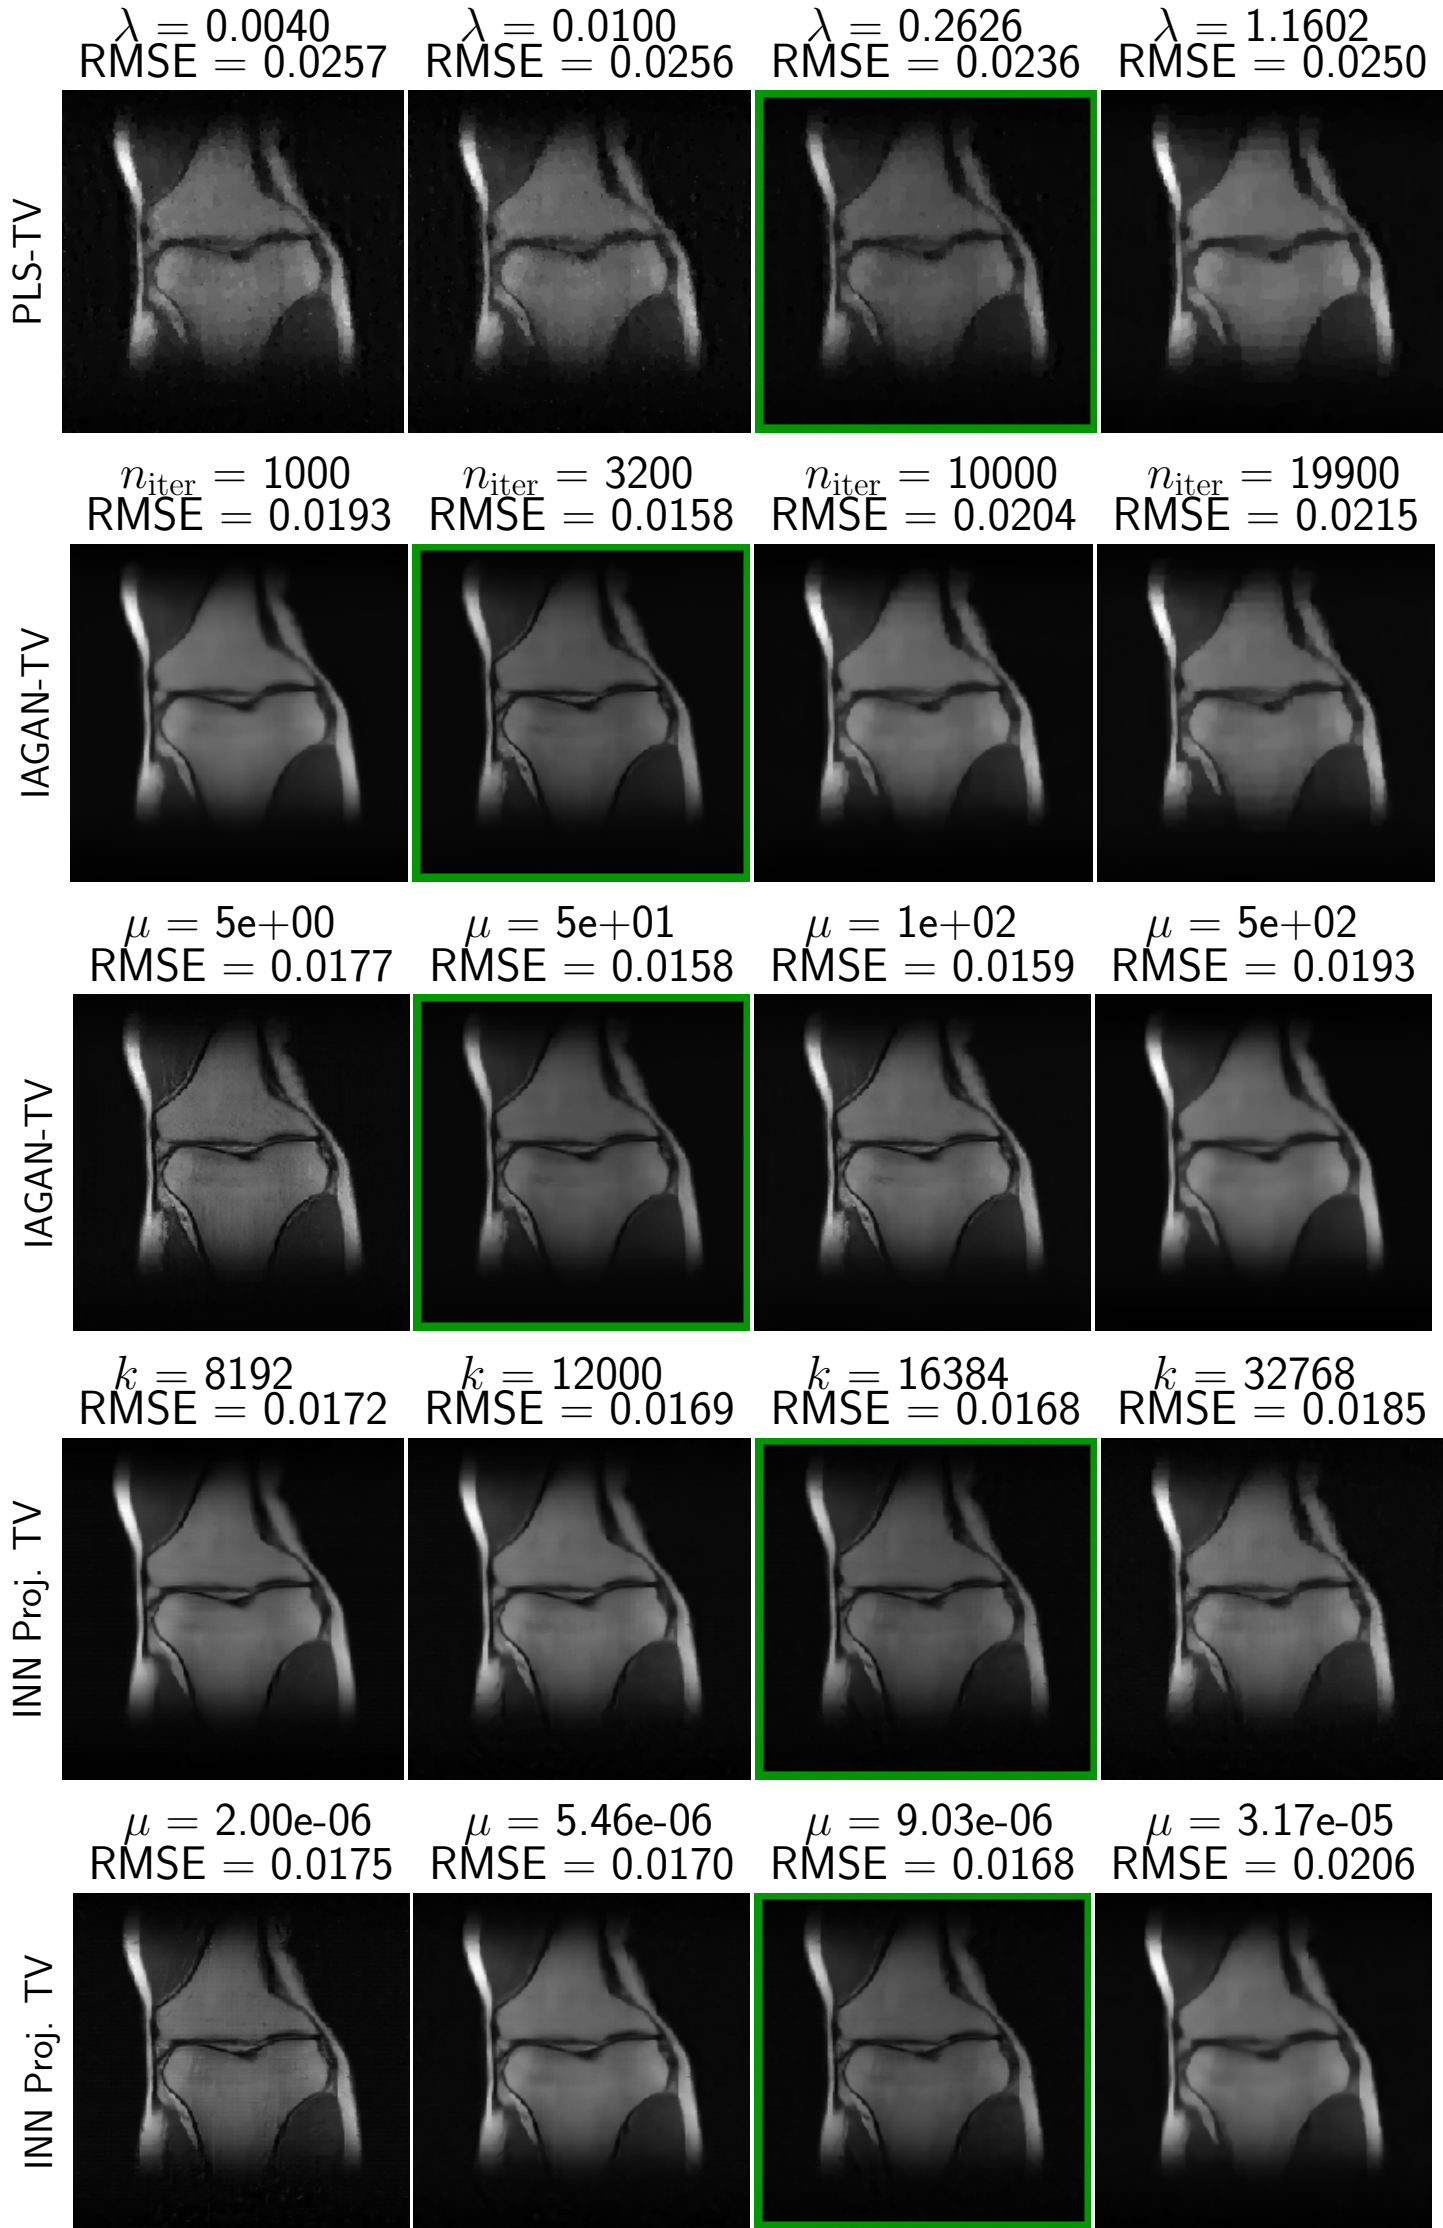 | 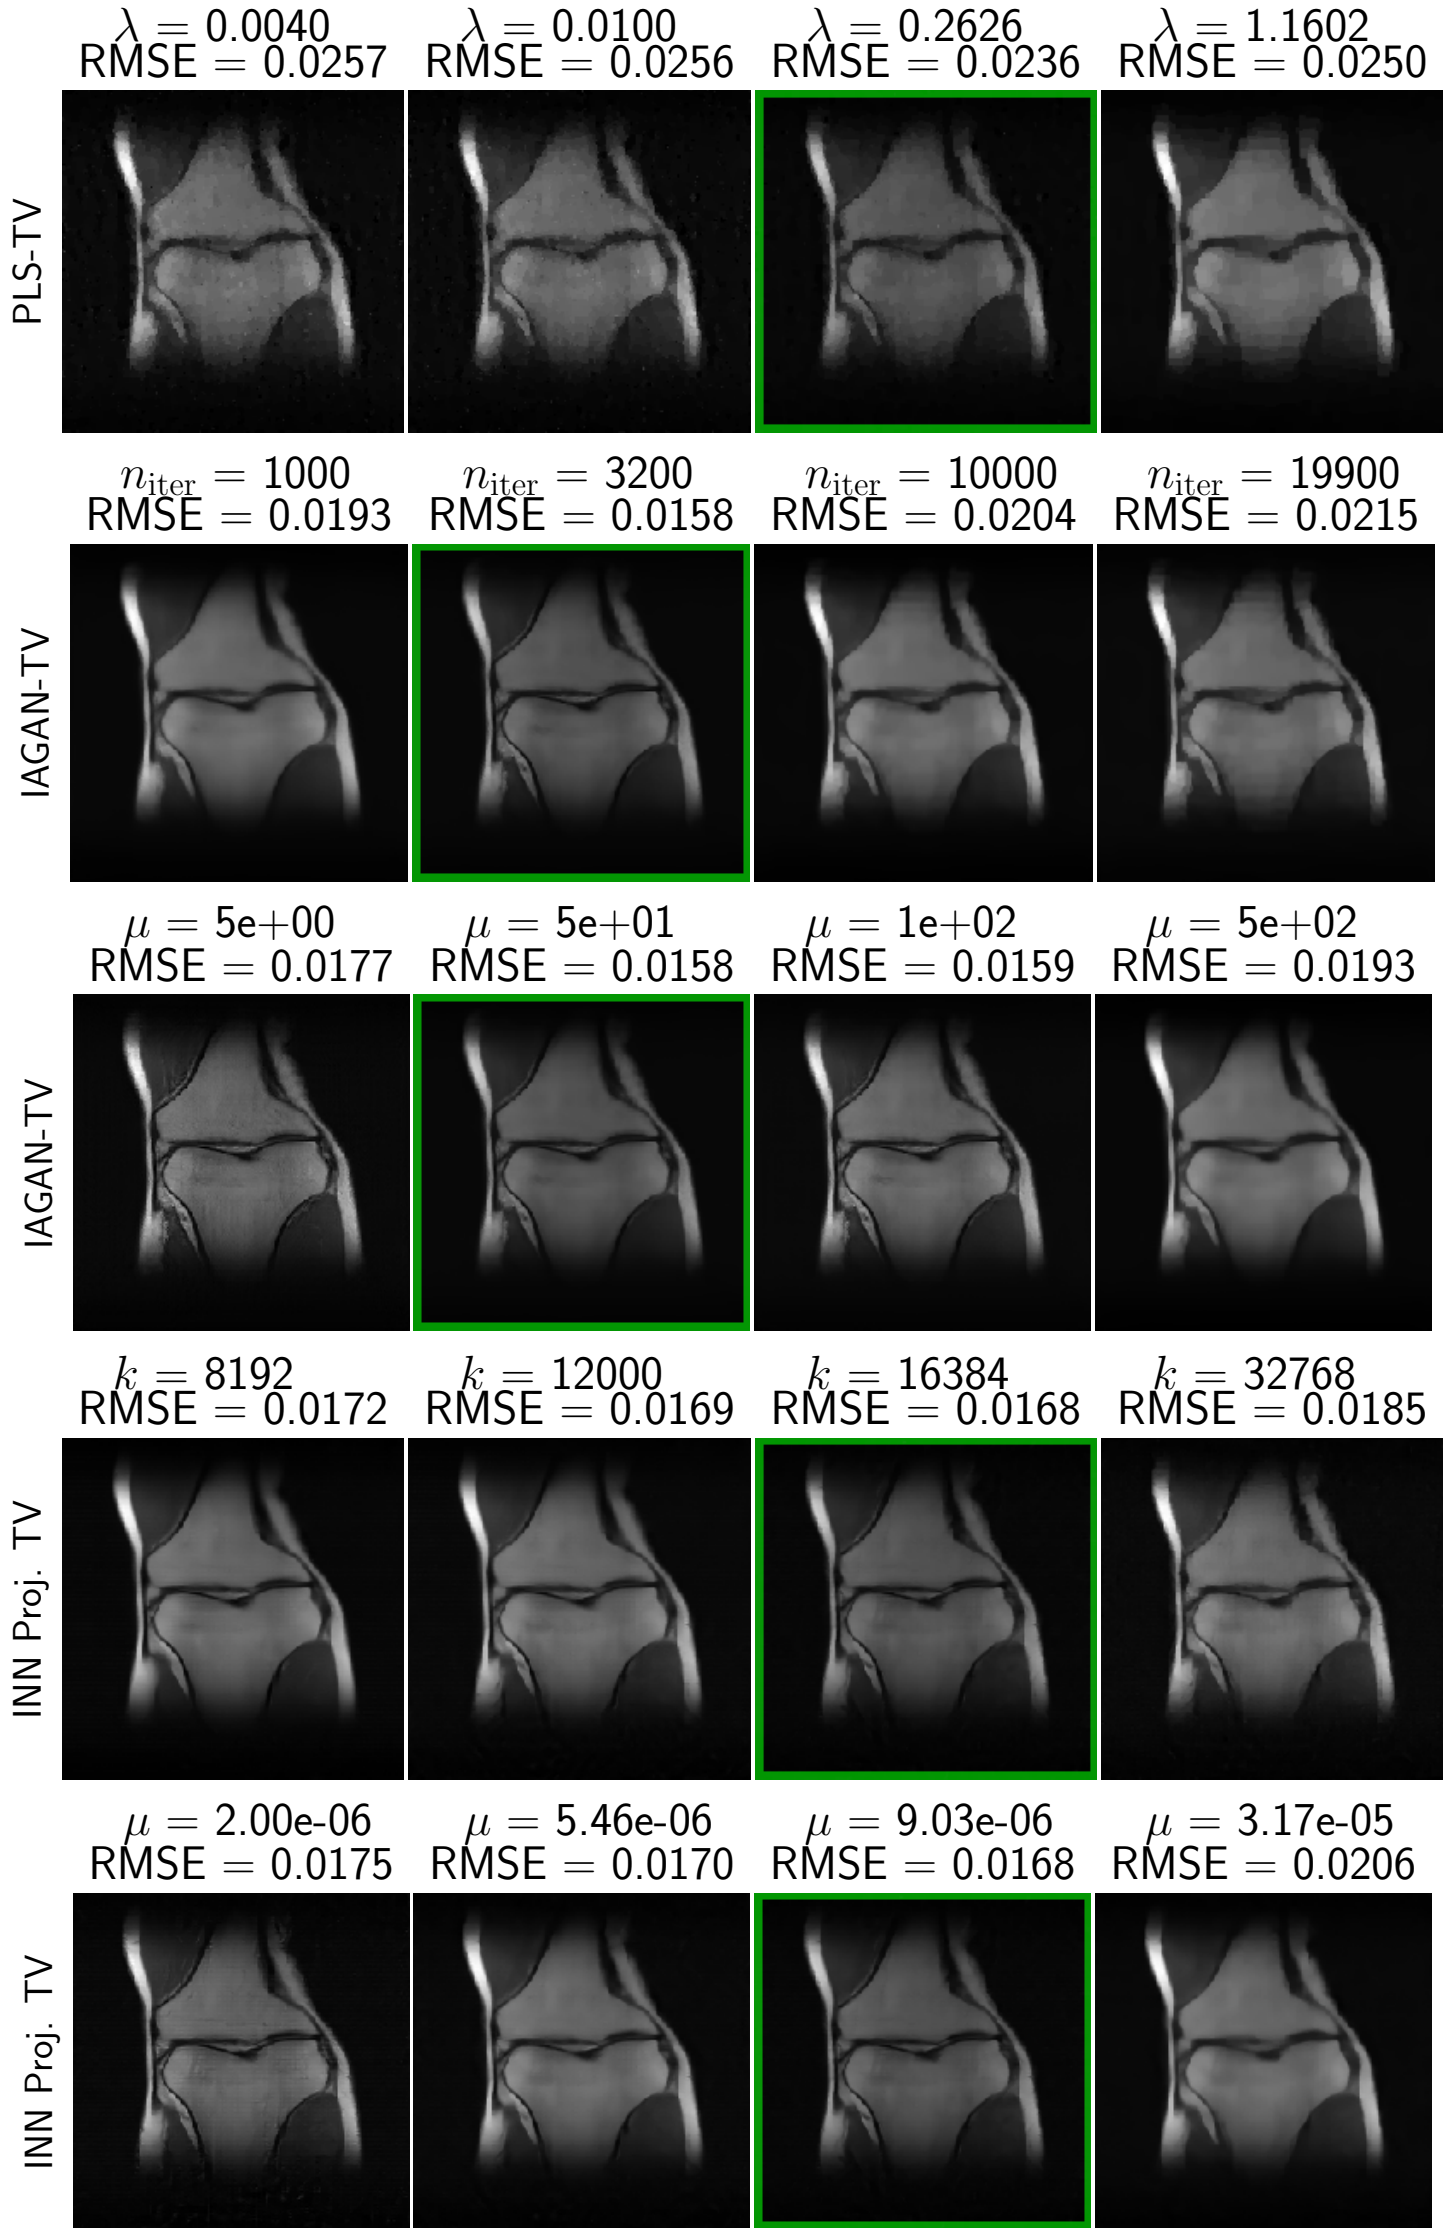 |
| INN Proj. TV | $\mu = 2.00e-06$<br>RMSE = 0.0175                                                   | $\mu = 5.46e-06$<br>RMSE = 0.0170                                                   | $\mu = 9.03e-06$<br>RMSE = 0.0168                                                    | $\mu = 3.17e-05$<br>RMSE = 0.0206                                                     |
|              | 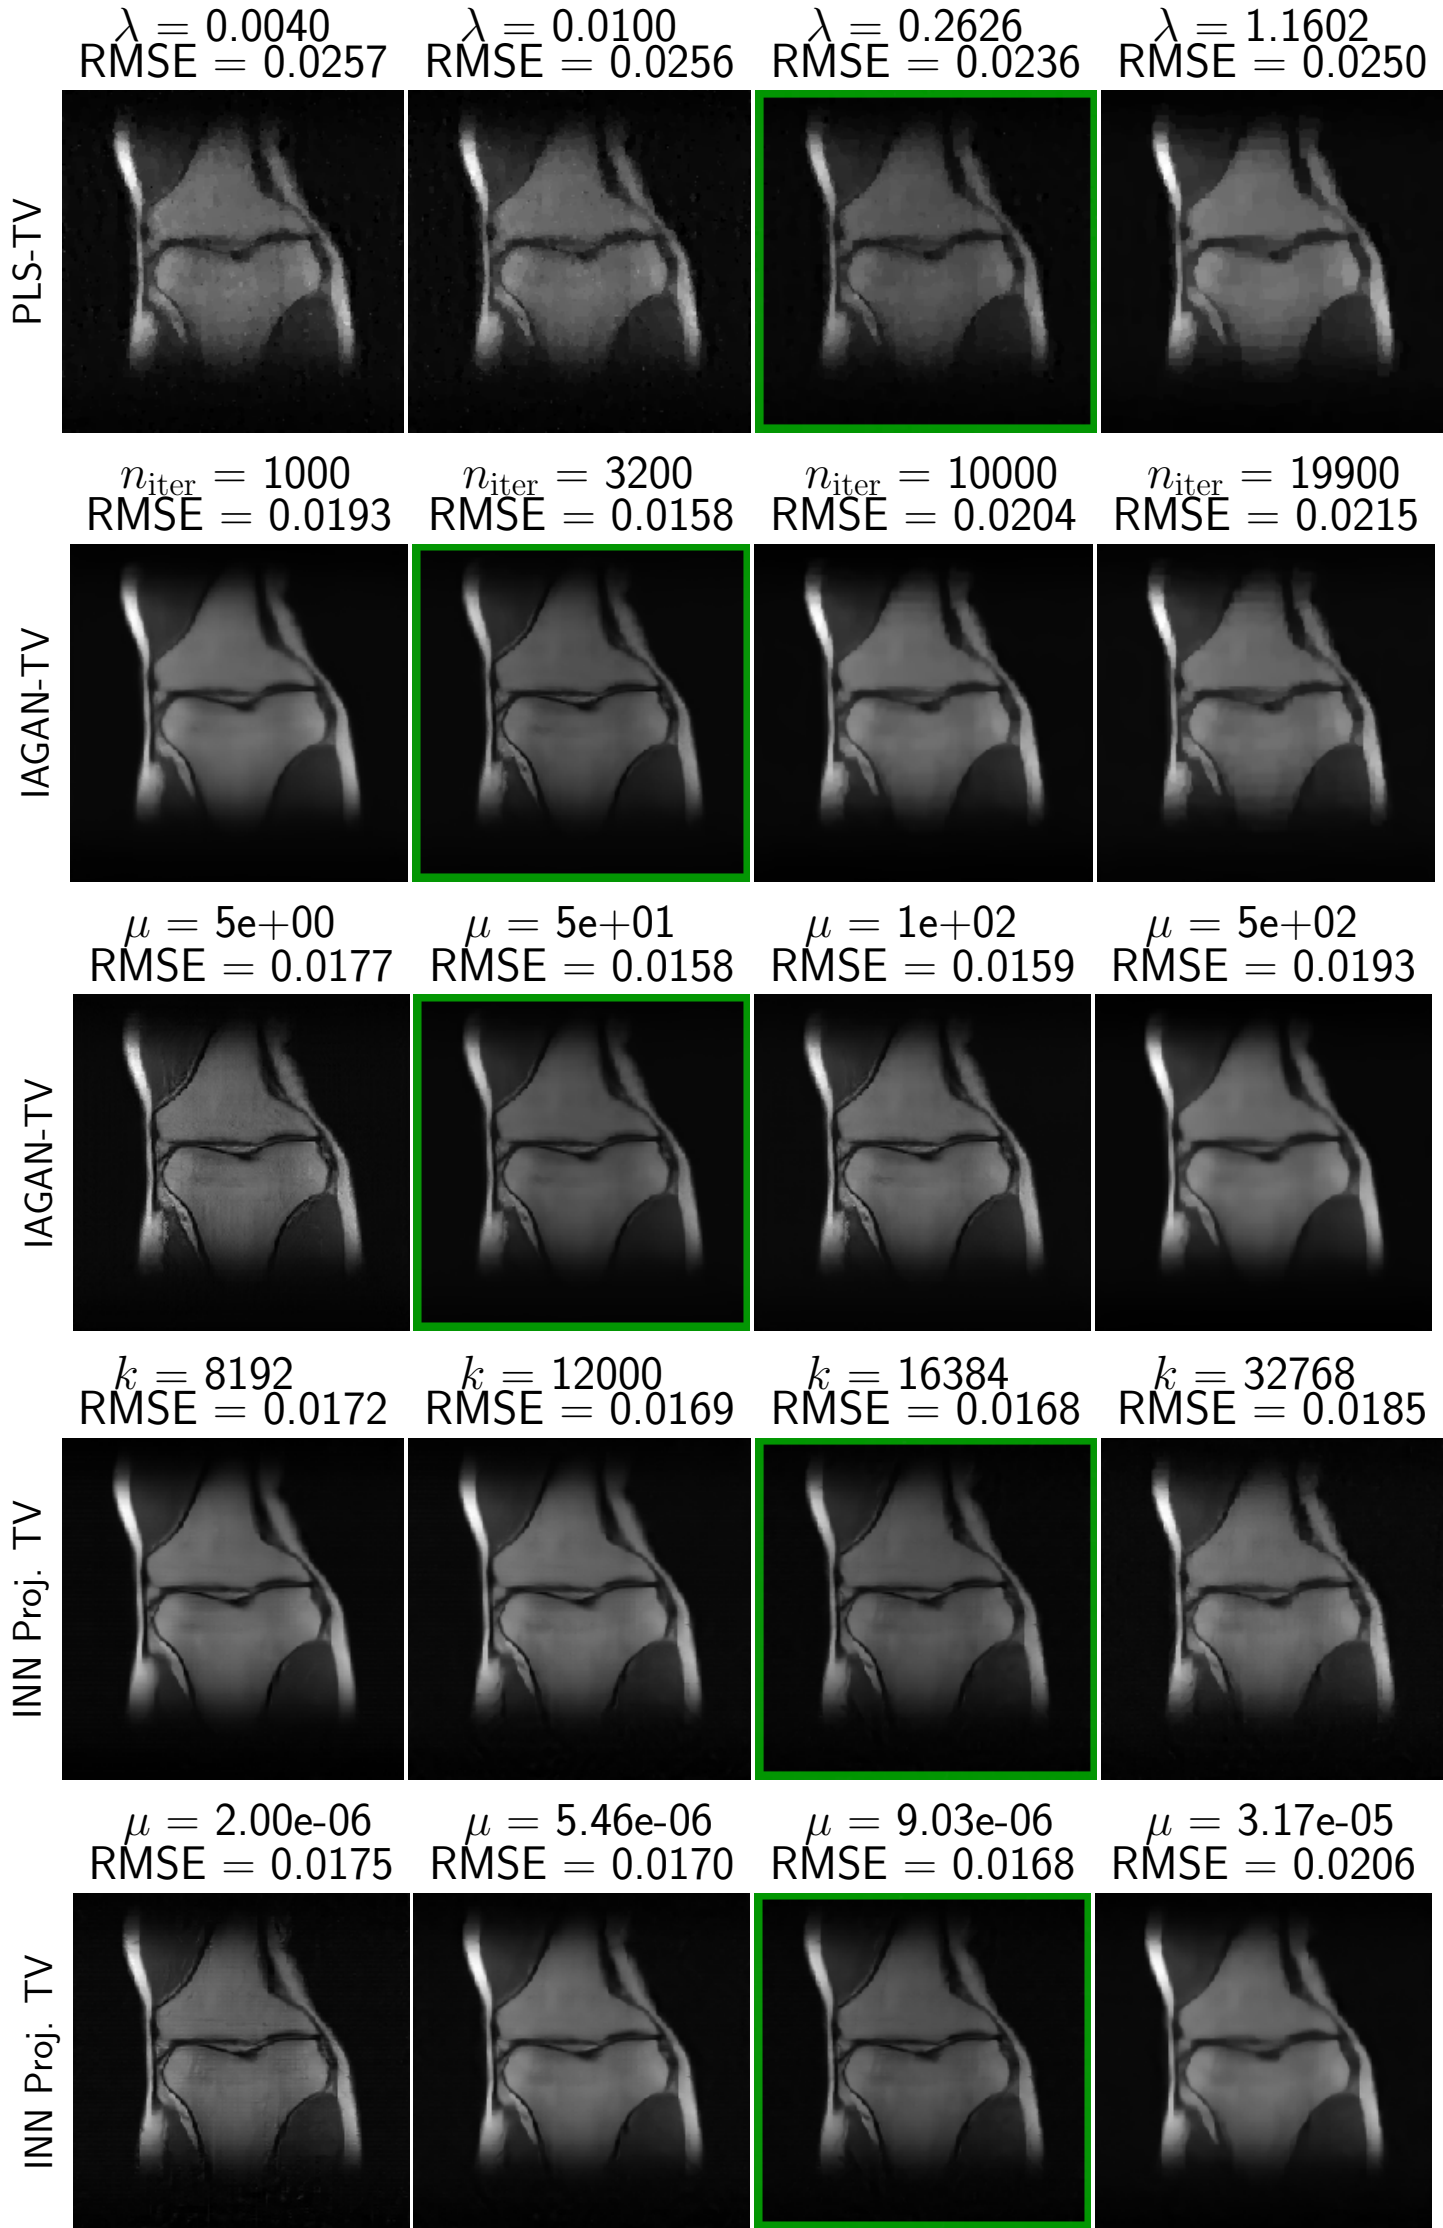 | 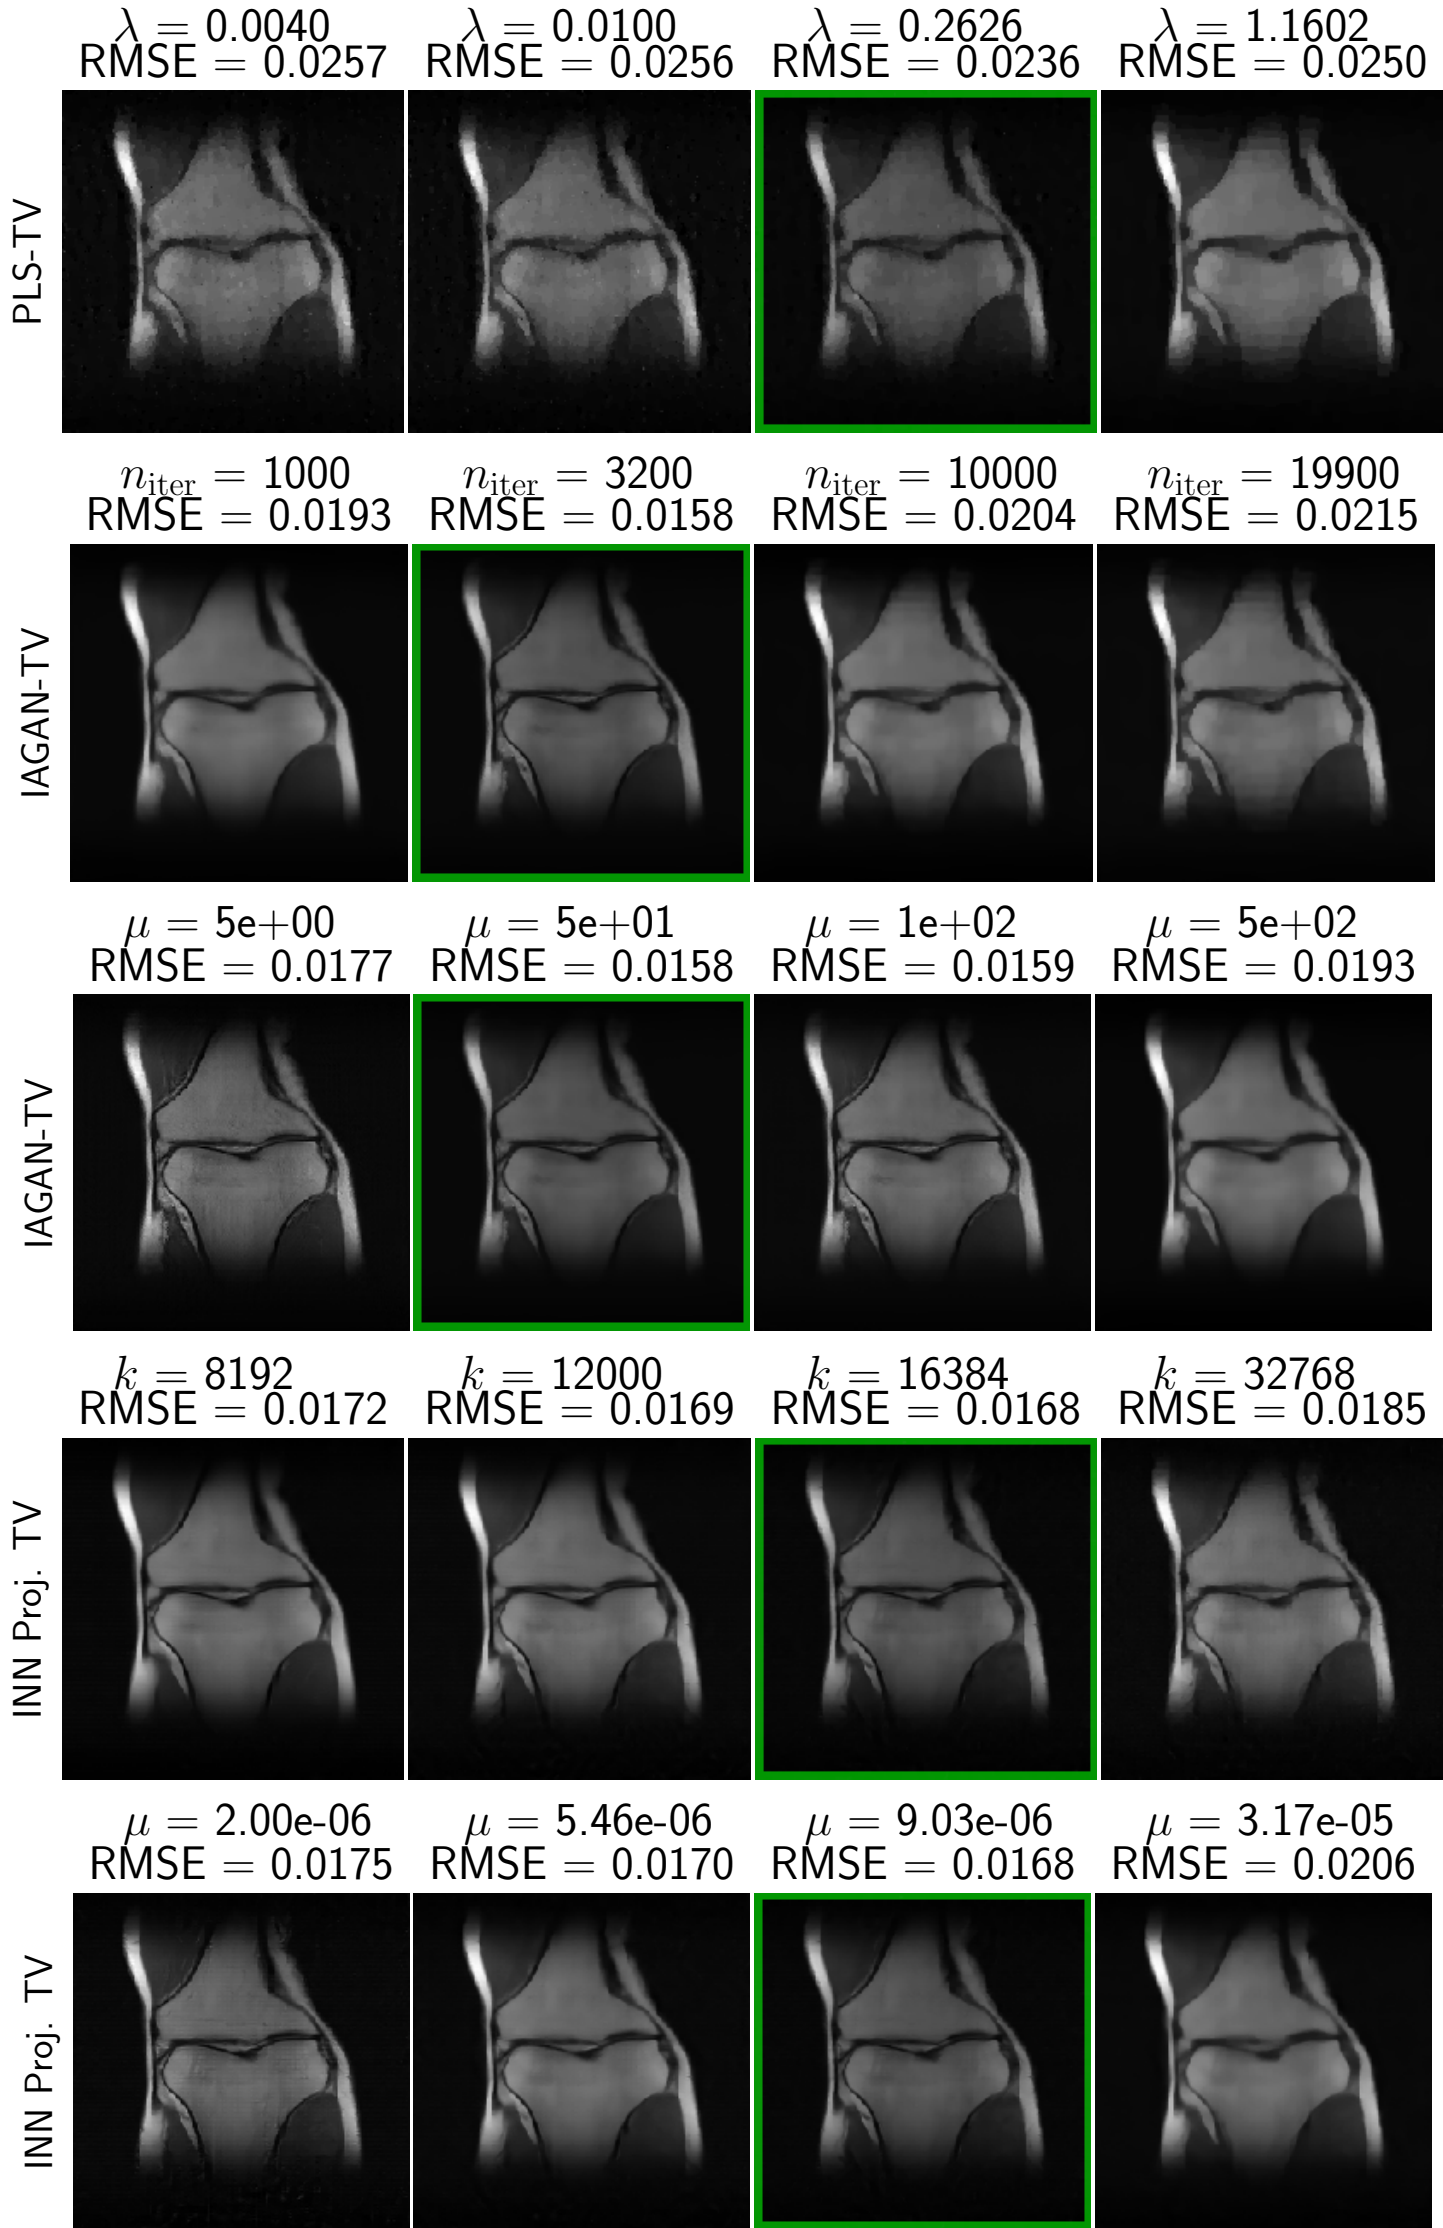 | 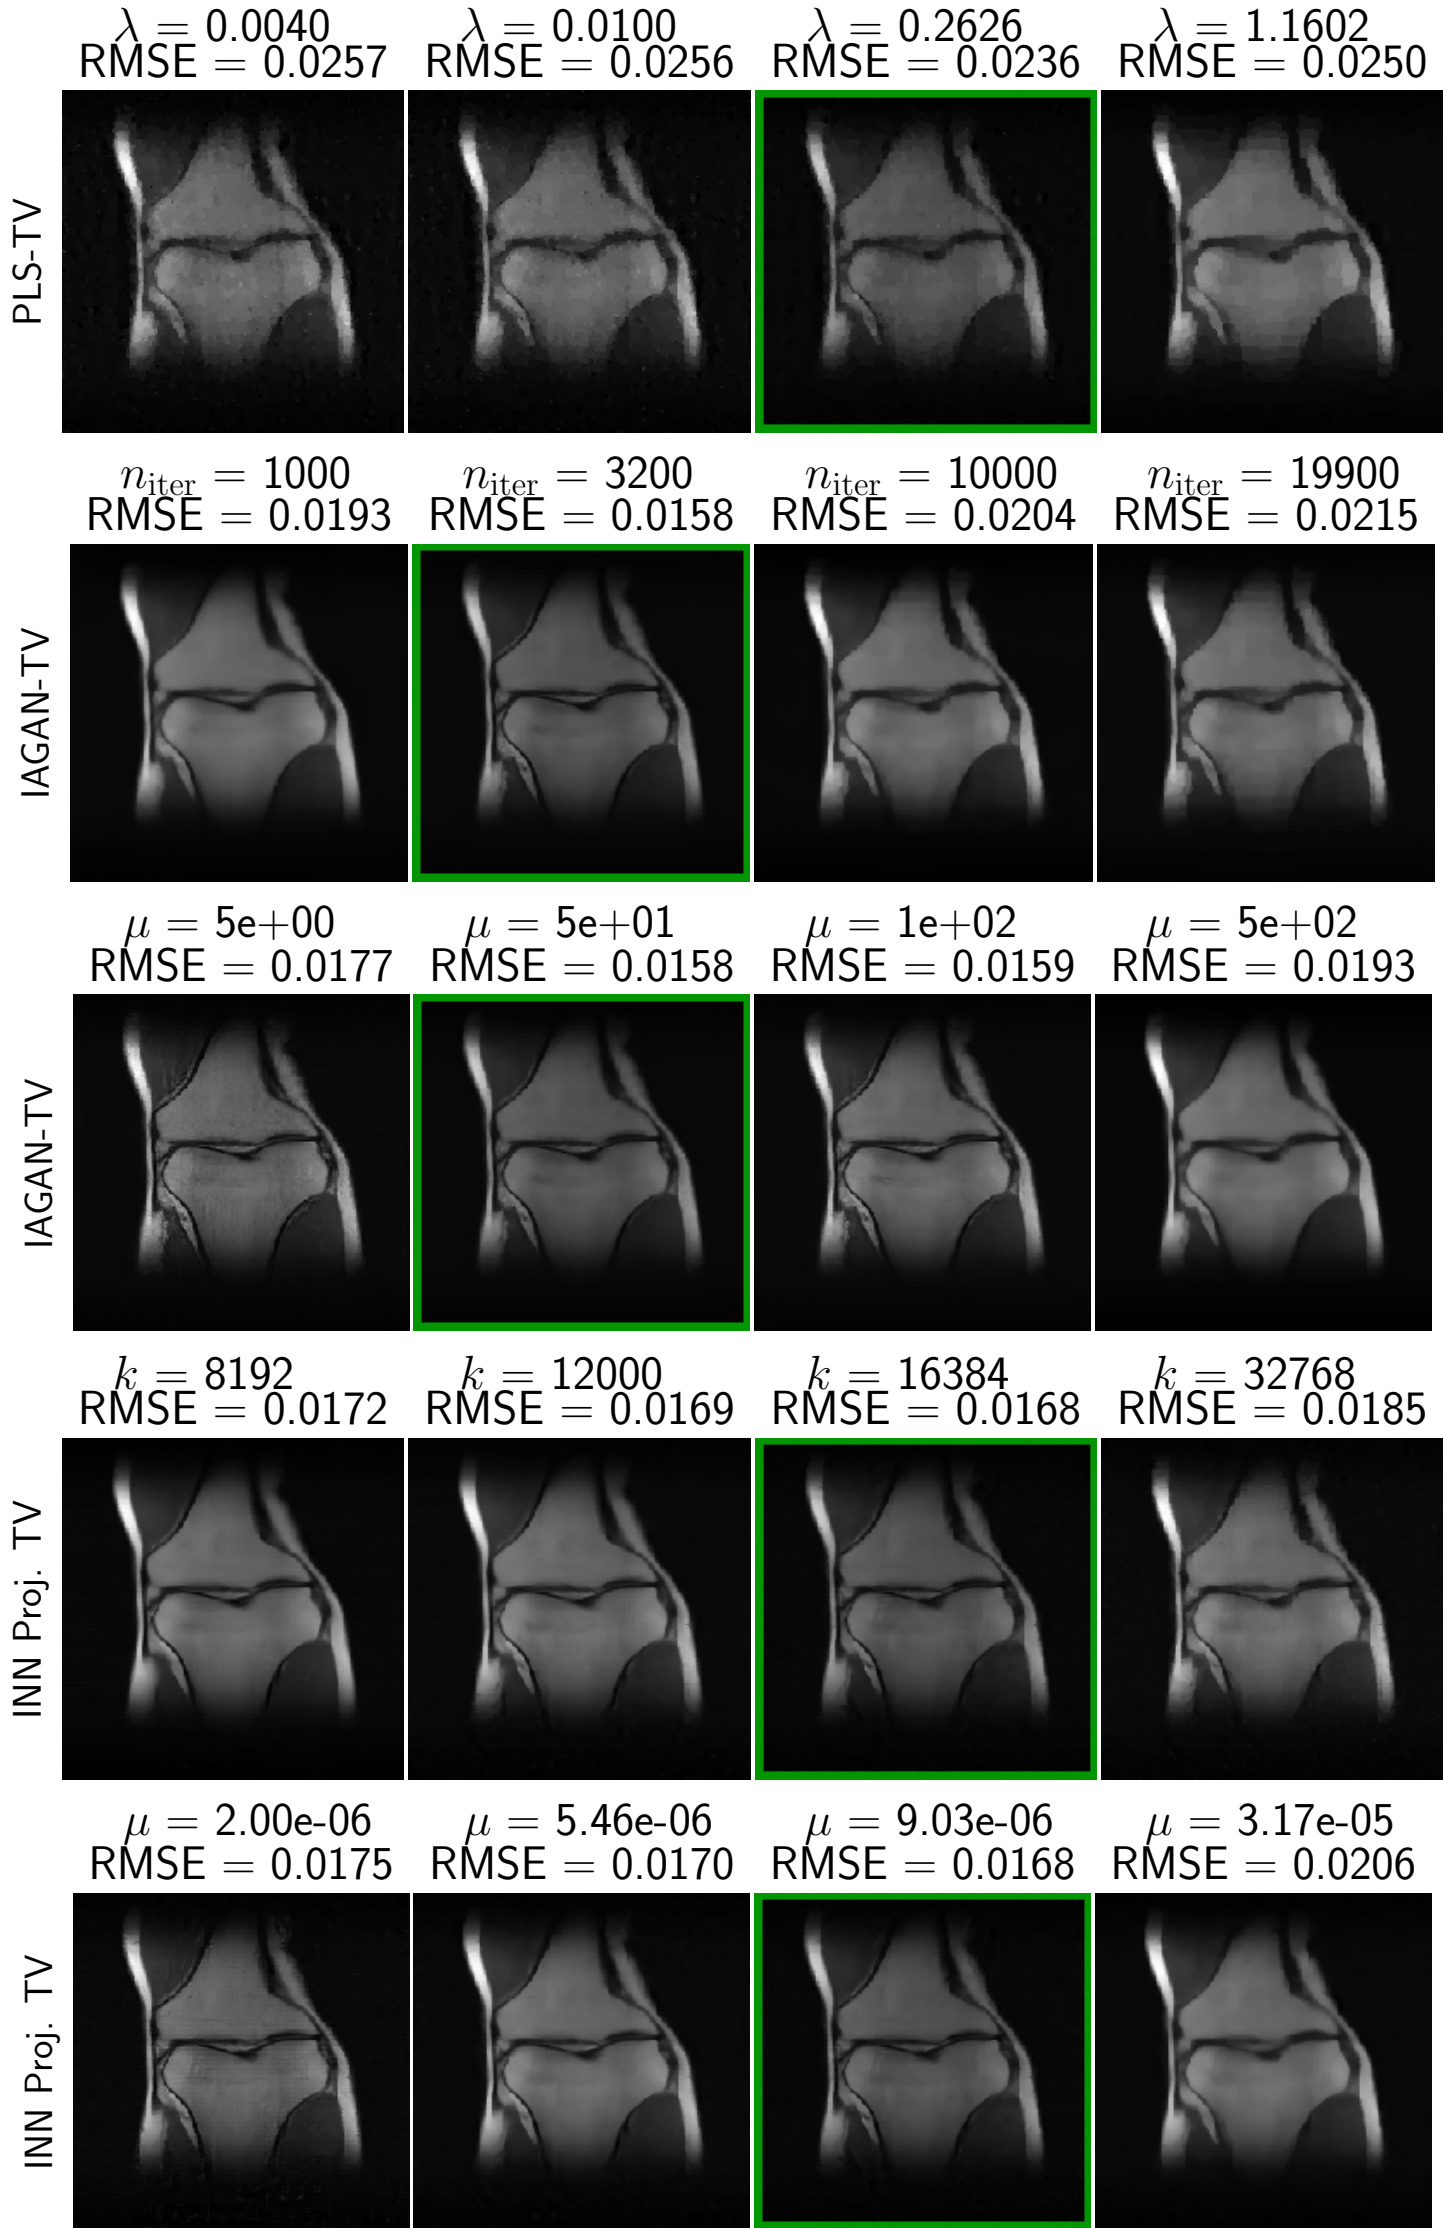 | 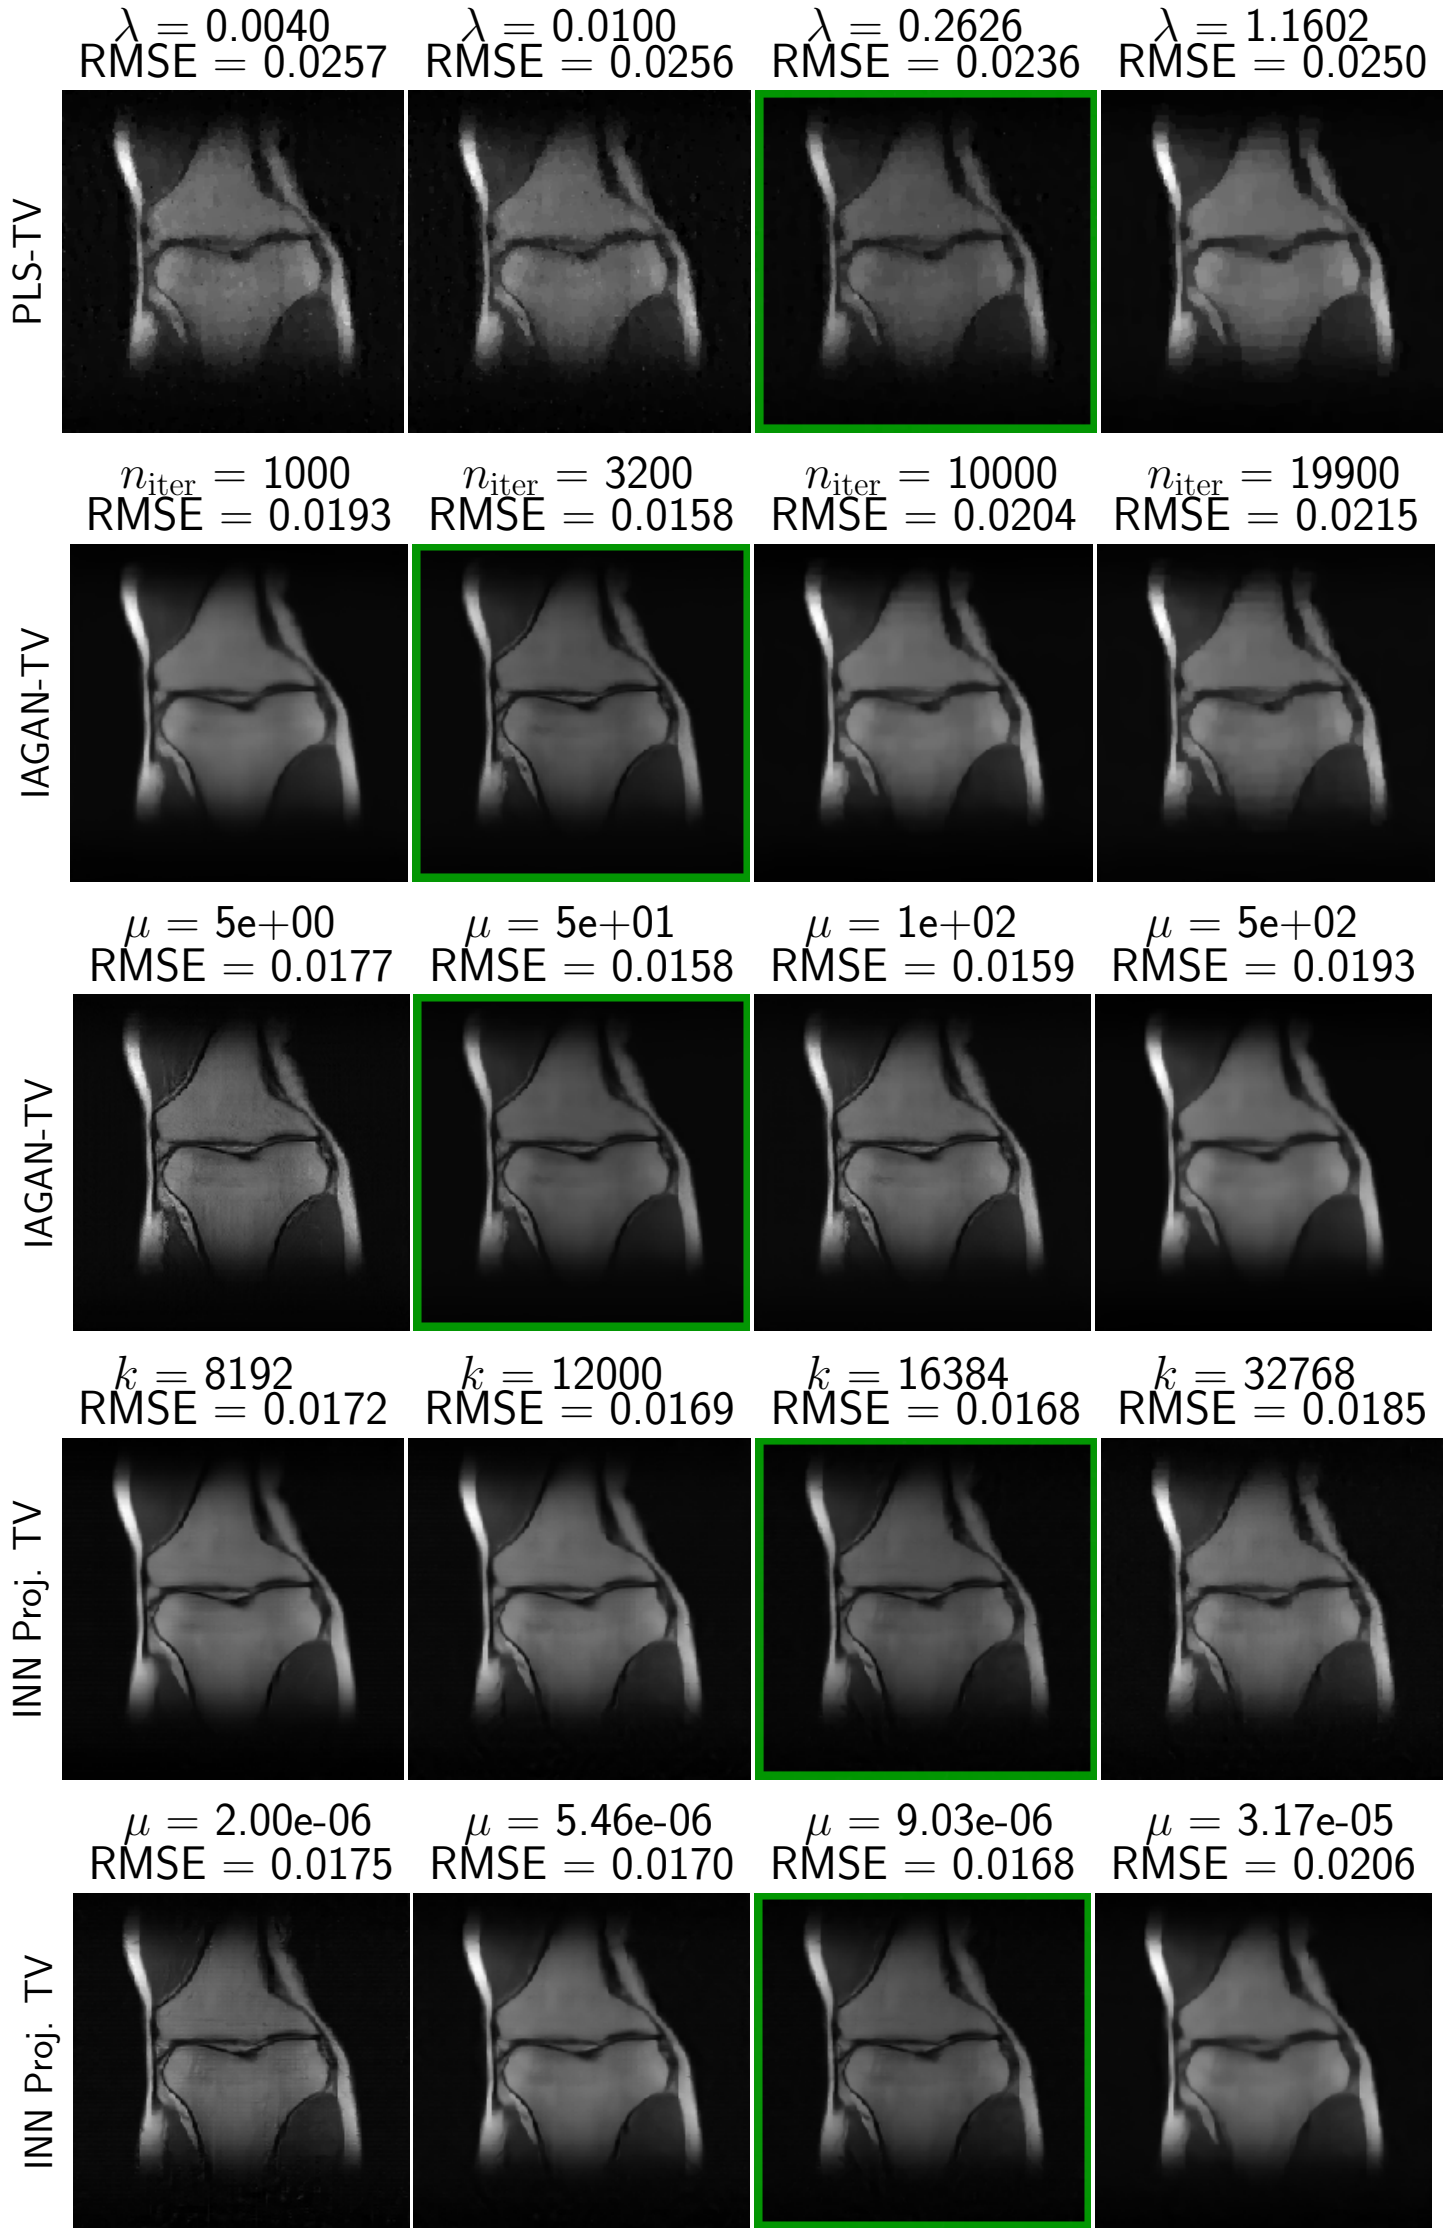 |

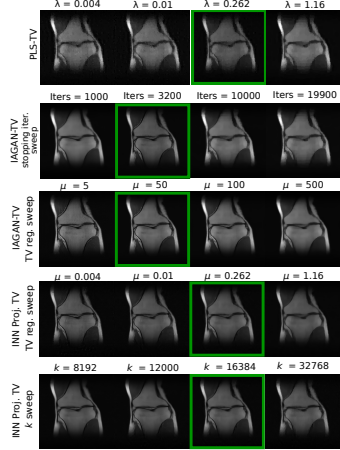

Supplement: Supplementary file 2 [file lamsweep_knee20x.pdf]
